# Supplementary material for: Techno-economic optimization of hybrid steam-electric energy systems with excess heat utilization and reserve market participation
Source: arXiv:2506.14252 source file (2025-06-17)
Supplement: Supplementary file 1 [file sm.tex]

\documentclass{article}
\usepackage{amsmath, amsfonts, amssymb, siunitx, graphicx, setspace, subcaption, booktabs, hyperref}
\usepackage[separate-uncertainty=true]{siunitx}
\usepackage[top=2.25cm, bottom=2.25cm, left=2.54cm, right=2.54cm]{geometry}

\DeclareSIUnit{\gCOtwoeq}{gCO\textsubscript{2-eq}}
\DeclareSIUnit{\tCOtwoeq}{tCO\textsubscript{2-eq}}
\DeclareSIUnit{\Wh}{Wh}
\DeclareSIUnit{\month}{mo.}
\DeclareSIUnit{\day}{day}
\sisetup{per-mode=symbol}

\title{Supplementary material for "Techno-economic optimization of hybrid steam–electric energy systems with excess heat utilization and reserve market participation"}

\author{
  Olav Galteland, Jacob Hadler-Jacobsen, and Hanne Kauko \\
  \normalsize Department of Thermal Energy, SINTEF Energy Research, Norway
}

\begin{document}
\maketitle
This supplementary material provides additional figures to support the findings presented in the main article, "Techno-economic optimization of hybrid steam–electric energy systems with excess heat utilization and reserve market participation". The results presented here offer results of the spot market electricity costs, grid tariffs, FCR market participation profits, and investment costs as the capacity of the electrode boiler, battery energy storage system (BESS), and steam accumulator capacities. These insights are intended to complement the techno-economic optimization results discussed in the main text.

The figures in this supplement follow the same format as figures in the main text where $\Delta$NPV is presented as a heat map as a function of electrode boiler, steam accumulator, and battery energy storage system (BESS) capacity, as well as the BESS C-rate. Bright colors (yellow) indicate high values, while dark colors (blue) indicate low values. The red star denotes the local optimum configuration, defined as the configuration with highest net present value, in each subfigure. Results are shown for both Norway and Germany. The color maps are consistent within each country across the subfigures, but not between countries. Configurations unable to meet the steam demand are marked with red hatched area.

\begin{figure}
    \centering
    \includegraphics[width=\linewidth]{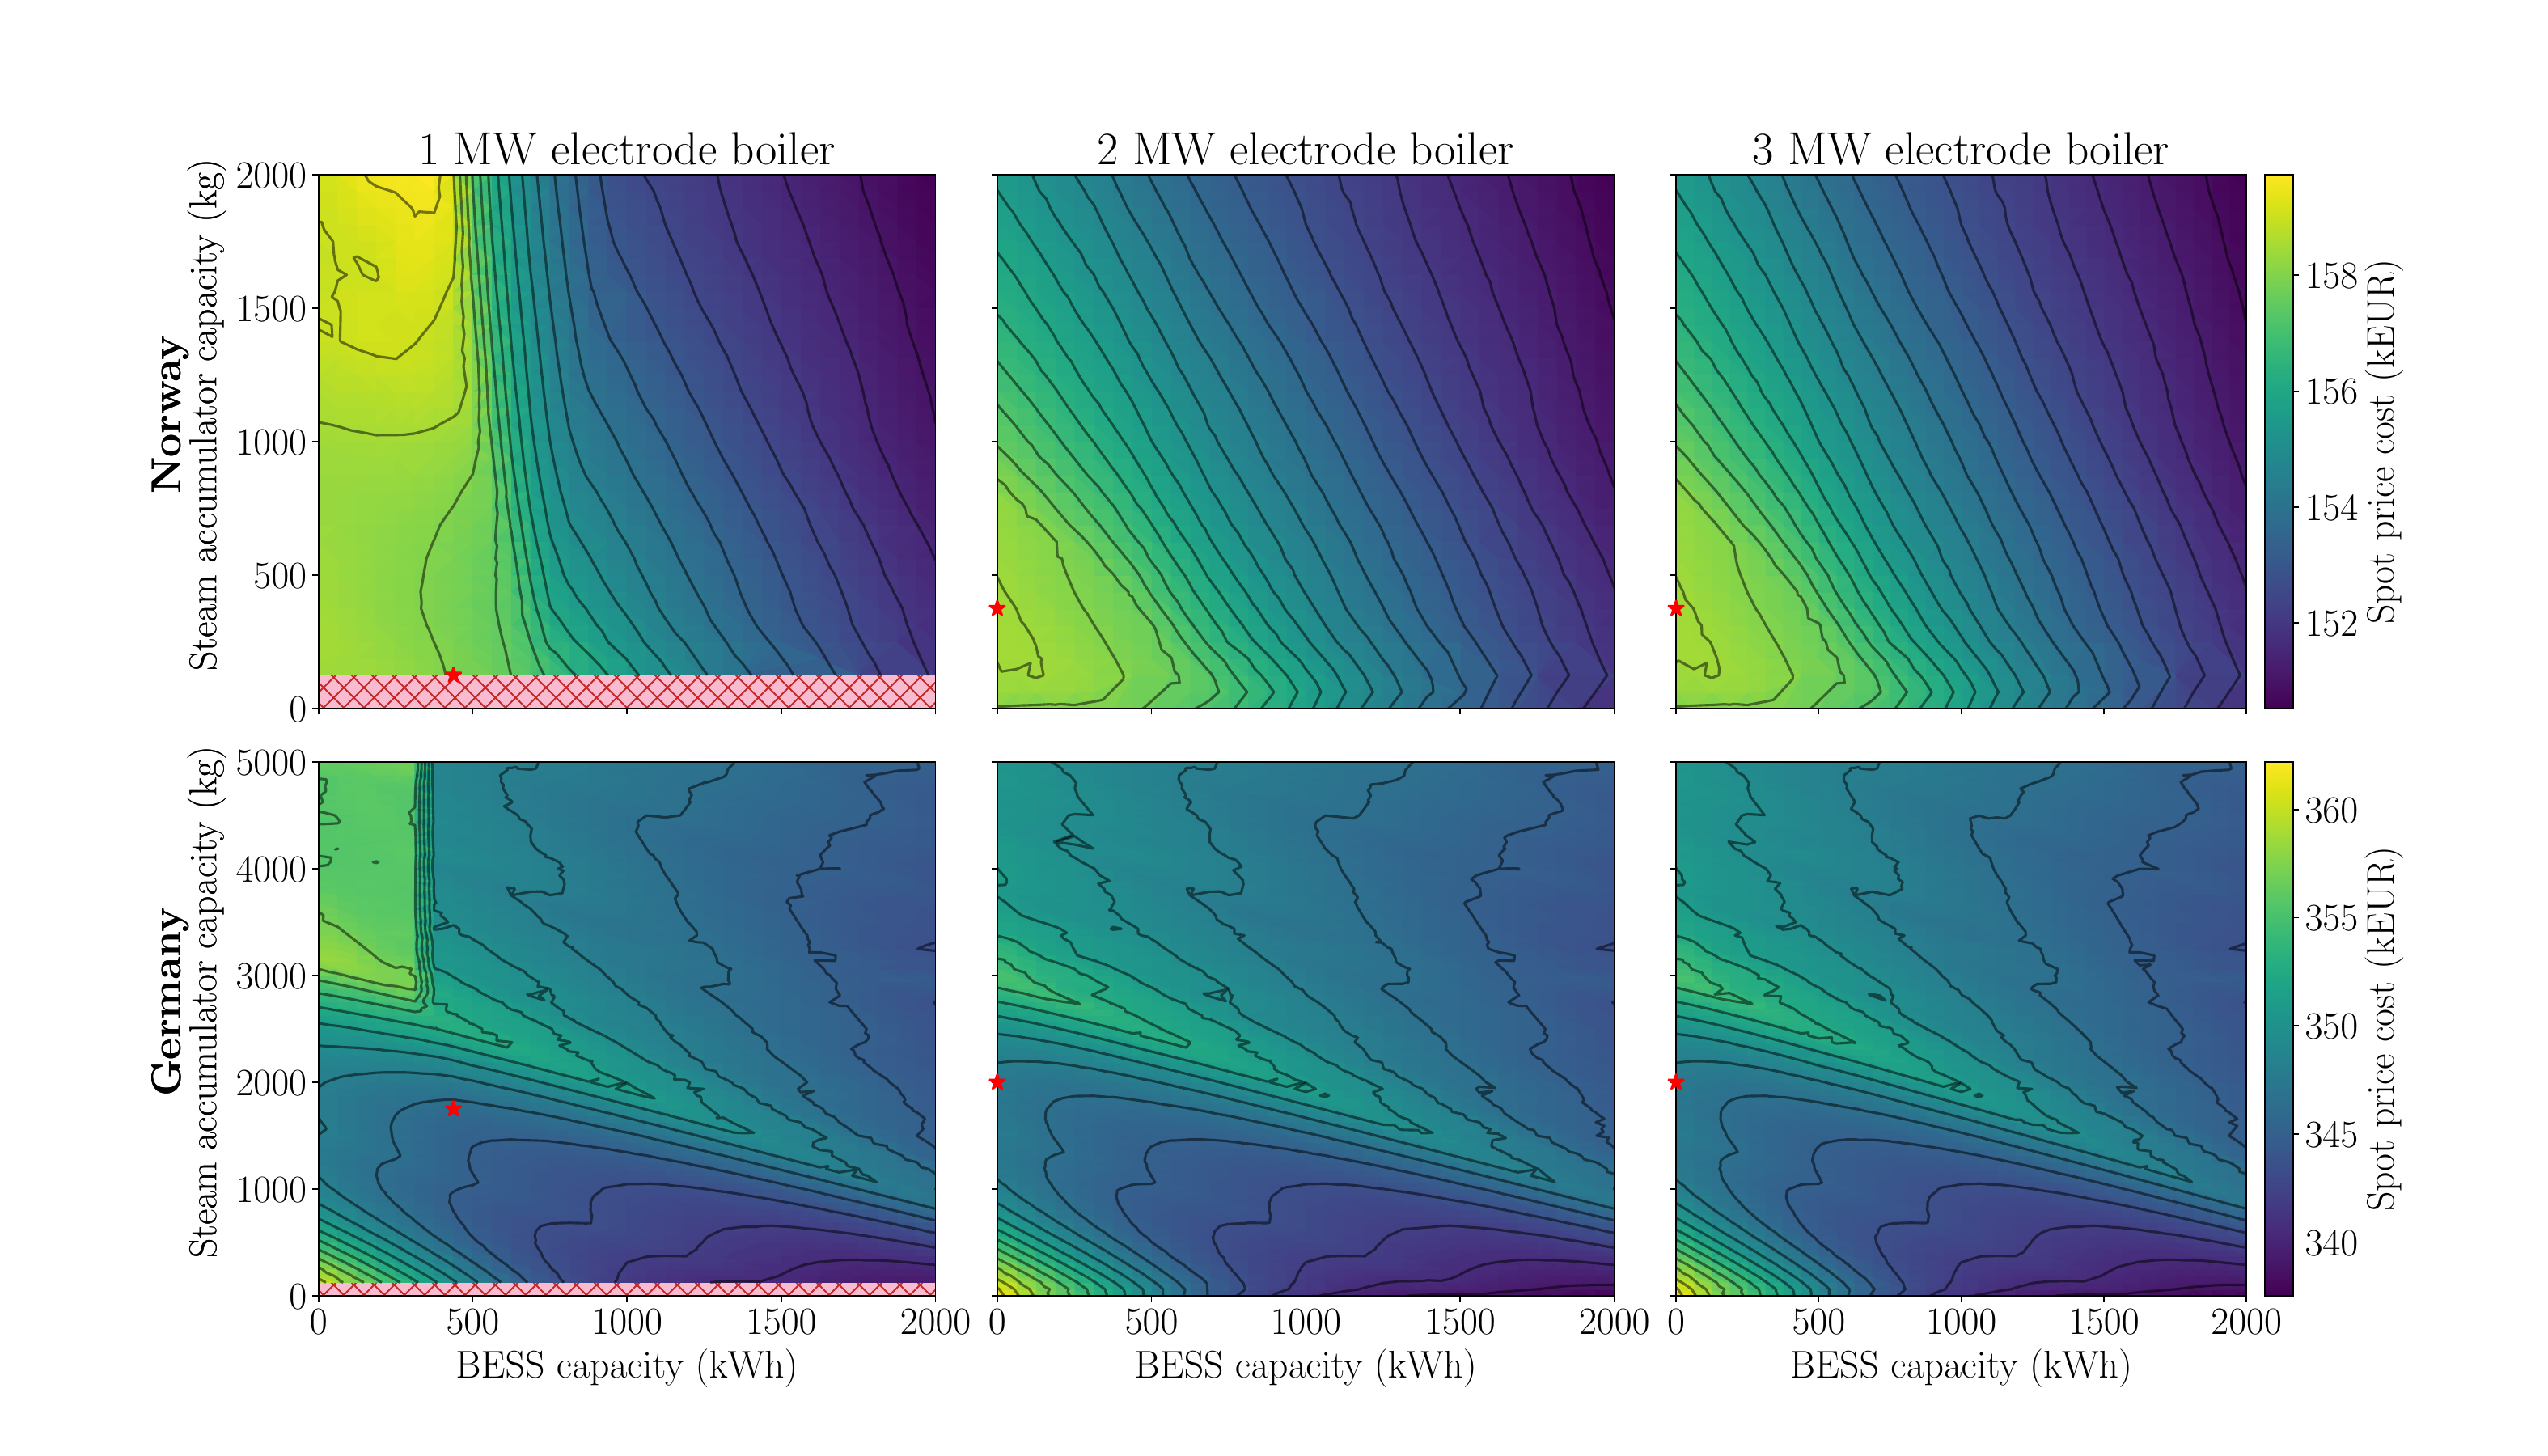}
    \caption{Heat map of the spot market electricity cost for Norway (top) and Germany (bottom) as a function of steam accumulator mass capacity and BESS capacity for three different electrode boiler capacities, (a) \SI{1}{\mega\watt}, (b) \SI{2}{\mega\watt}, an (c) \SI{3}{\mega\watt}. The red star indicates the maximum net present value for each capacity of electrode boiler.}
\end{figure}

\begin{figure}
    \centering
    \includegraphics[width=\linewidth]{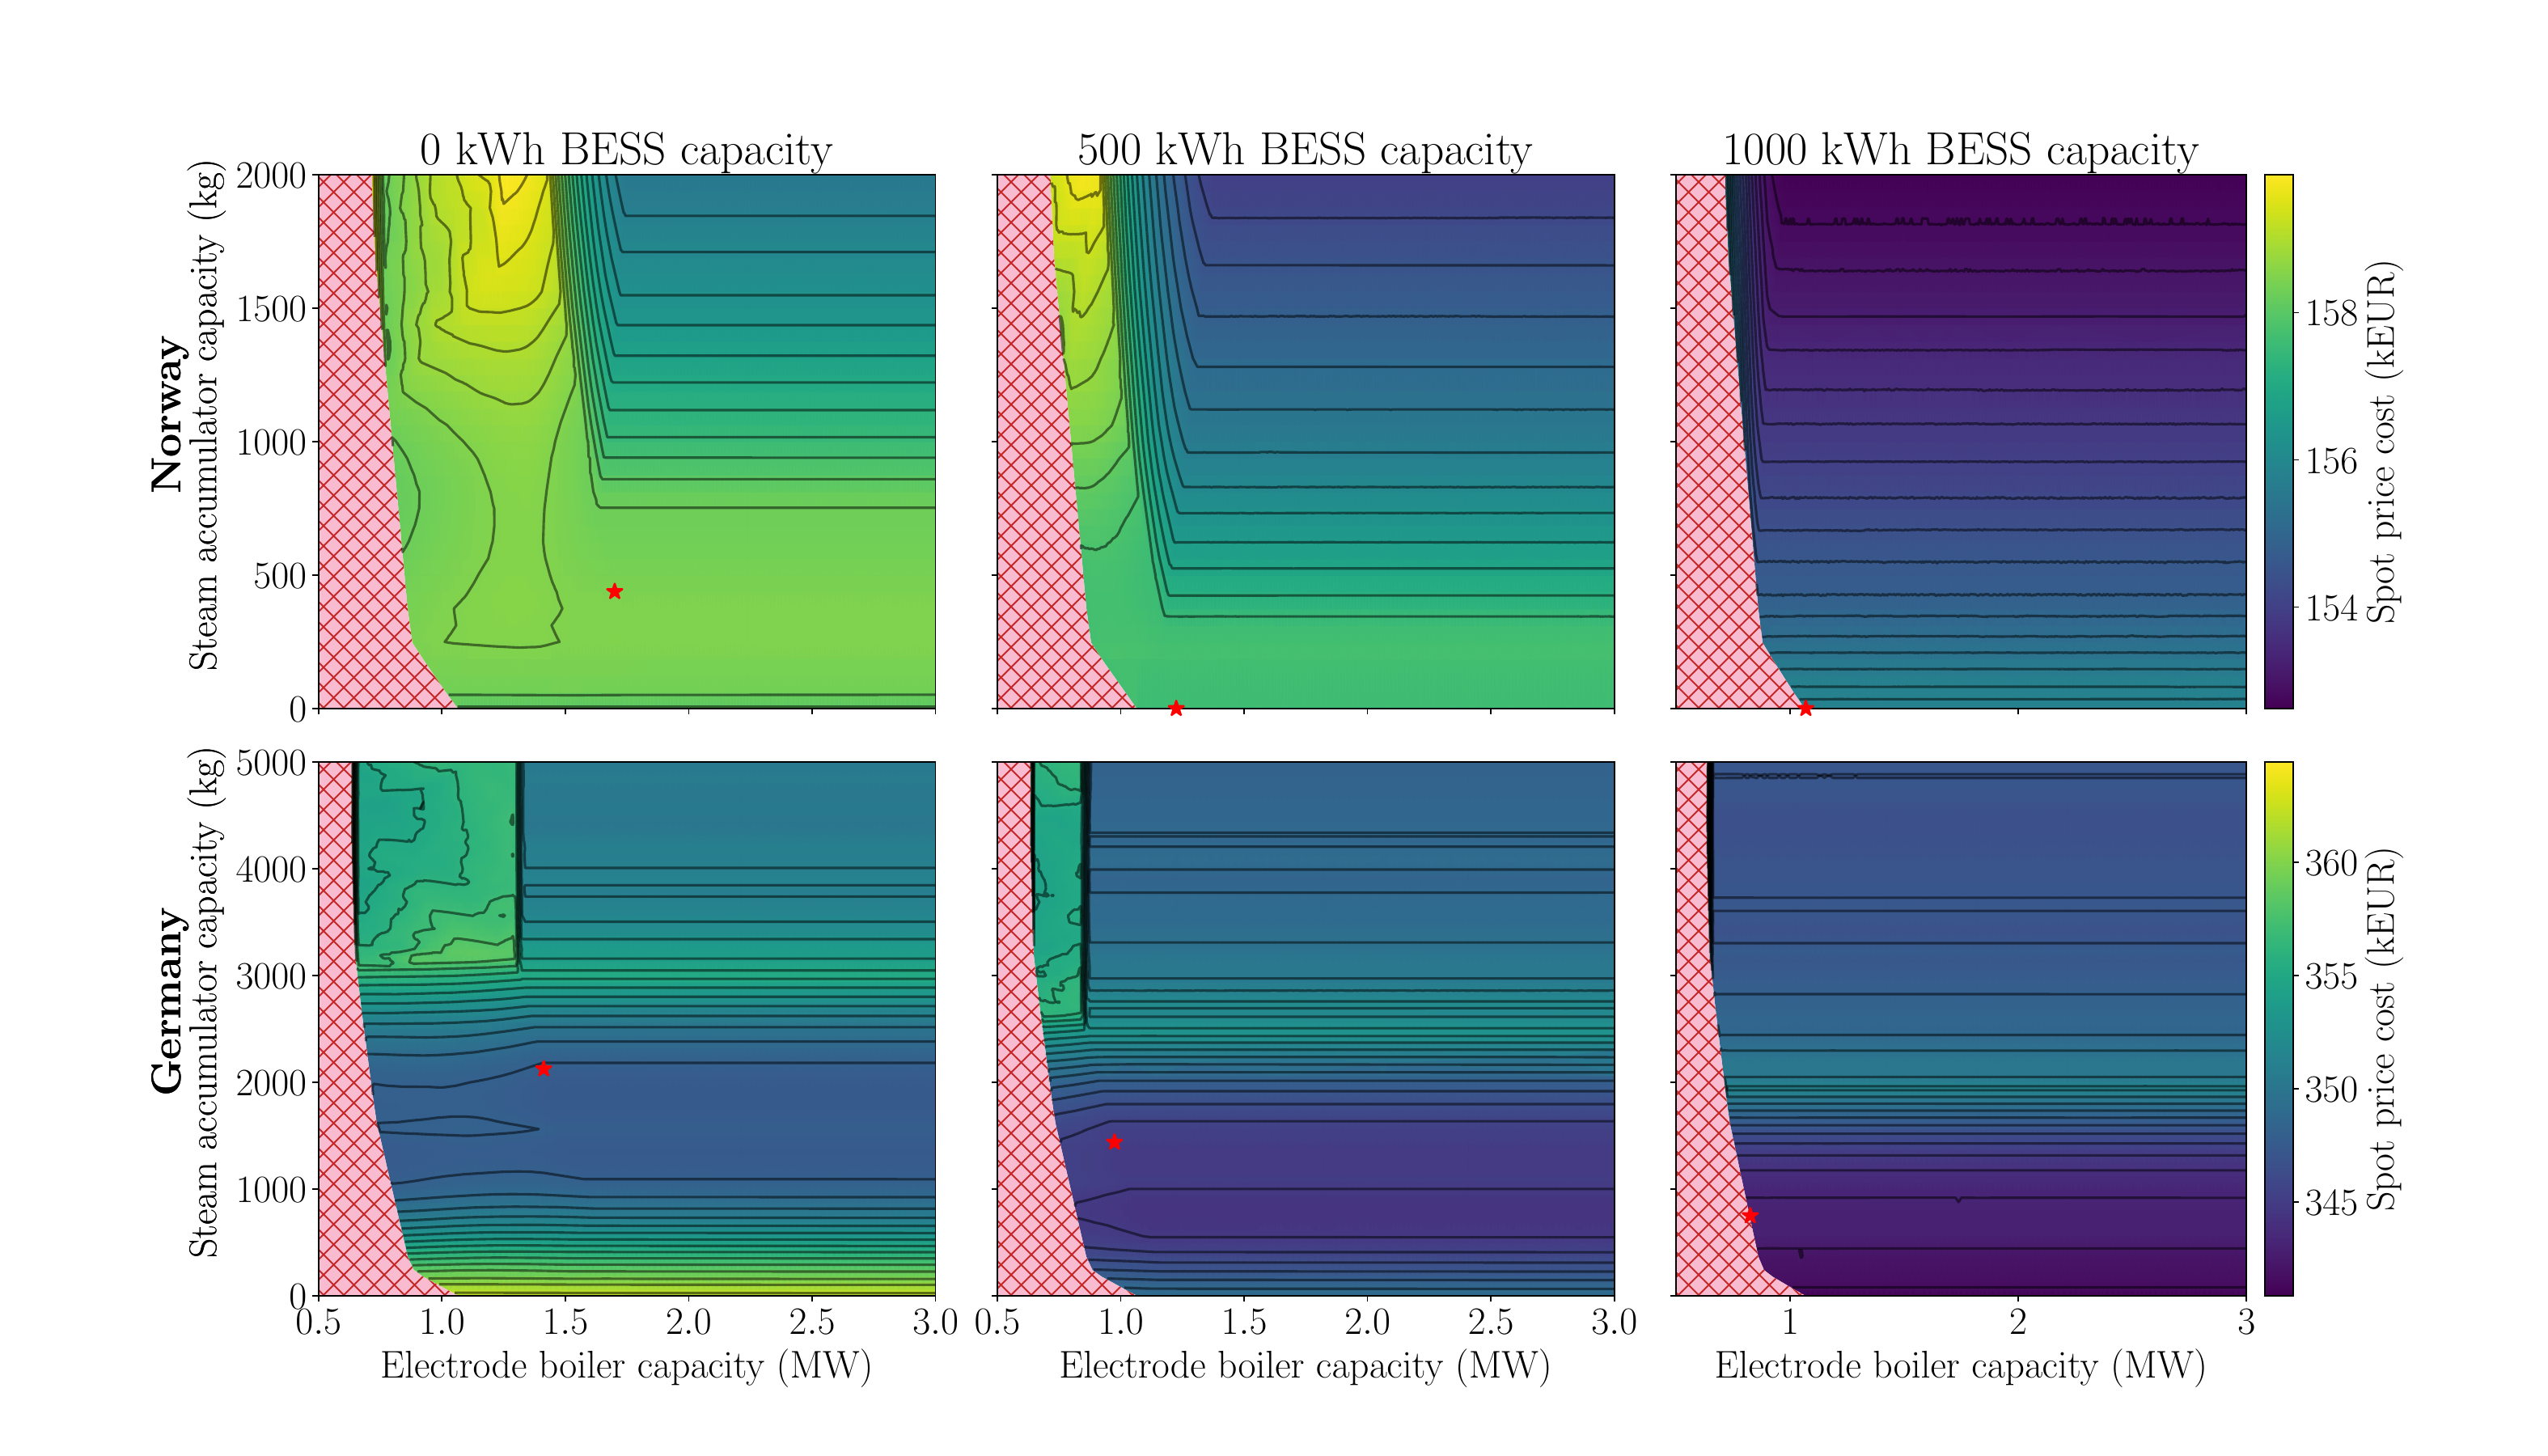}
    \caption{Heat map of the spot market electricity cost for Norway (top) and Germany (bottom) as a function of steam accumulator mass capacity and electrode boiler for three different BESS capacities, (a) \SI{0}{\kilo\Wh}, (b) \SI{500}{\kilo\Wh}, an (c) \SI{1000}{\kilo\Wh} and C-rate of 0.9. The red star indicates the maximum net present value for each capacity of electrode boiler.}
\end{figure}

\begin{figure}
    \centering
    \includegraphics[width=\linewidth]{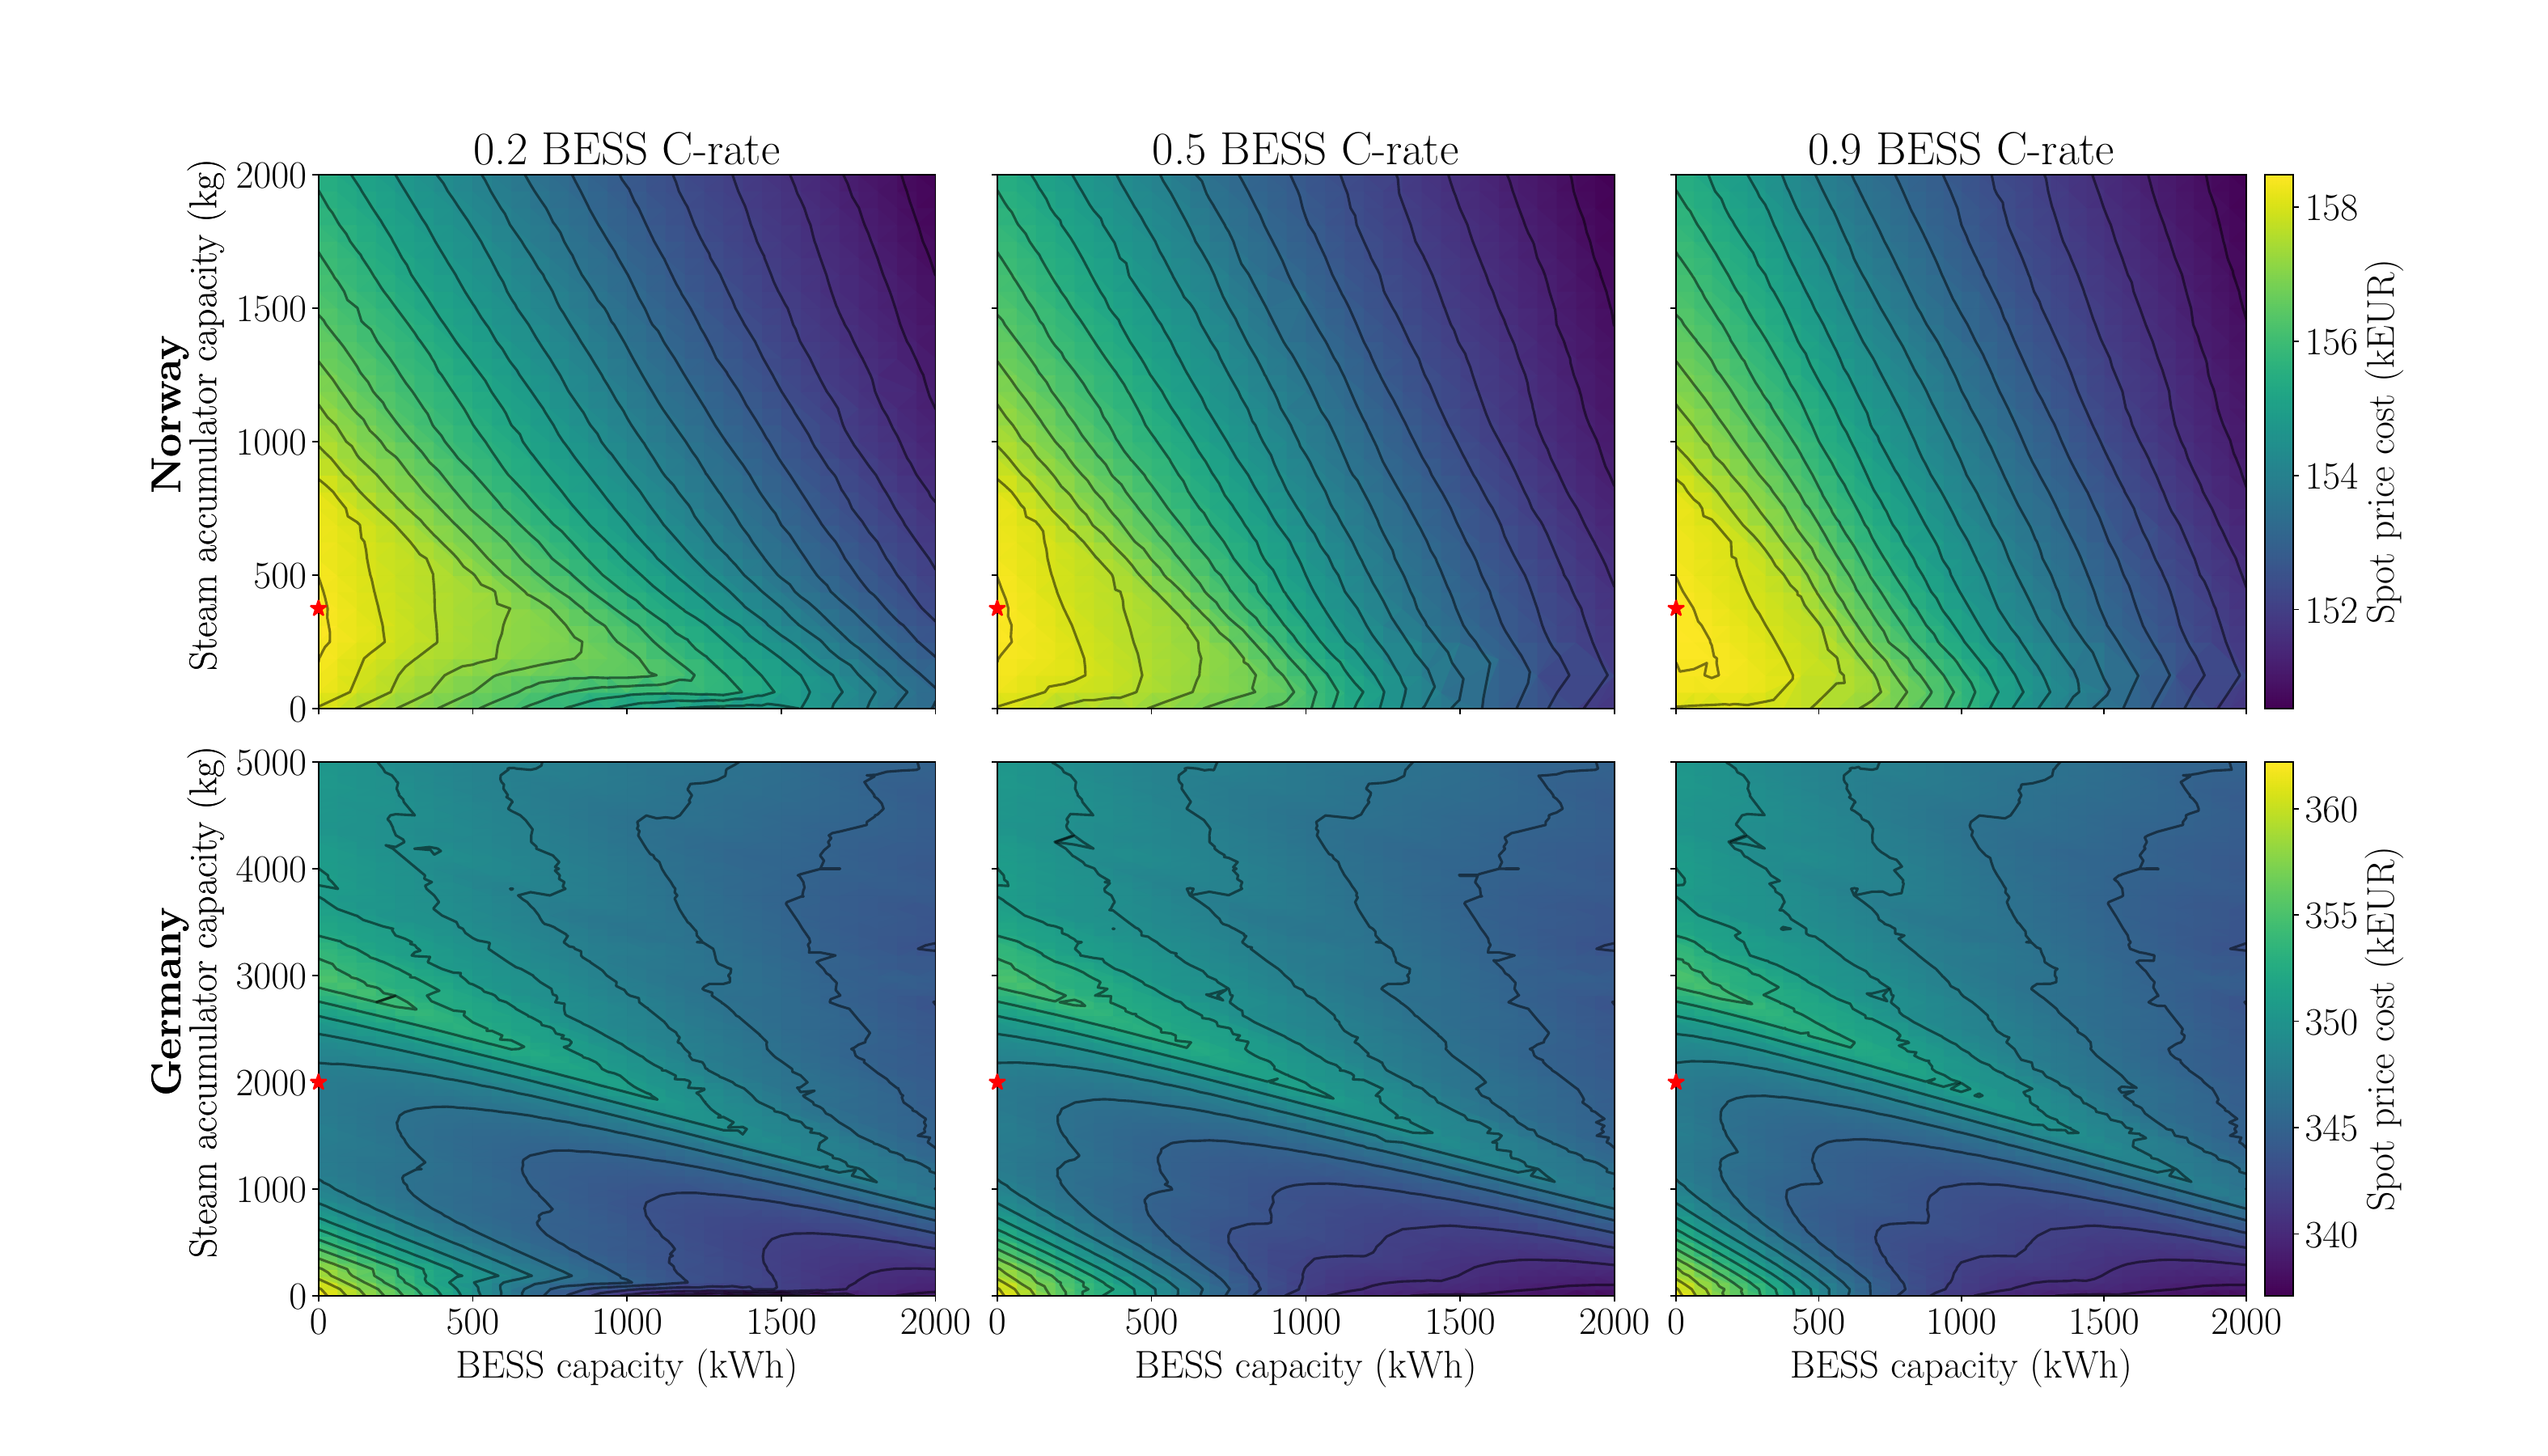}
    \caption{Heat map of the spot market electricity cost for Norway (top) and Germany (bottom) as a function of steam accumulator mass capacity and BESS capacity for electrode boiler capacity of \SI{2}{\mega\watt} and three different BESS C-rates (a) 0.2, (b) 0.5, and (c) 1. The red star indicates the maximum net present value for each capacity of electrode boiler.}
\end{figure}

\begin{figure}
    \centering
    \includegraphics[width=\linewidth]{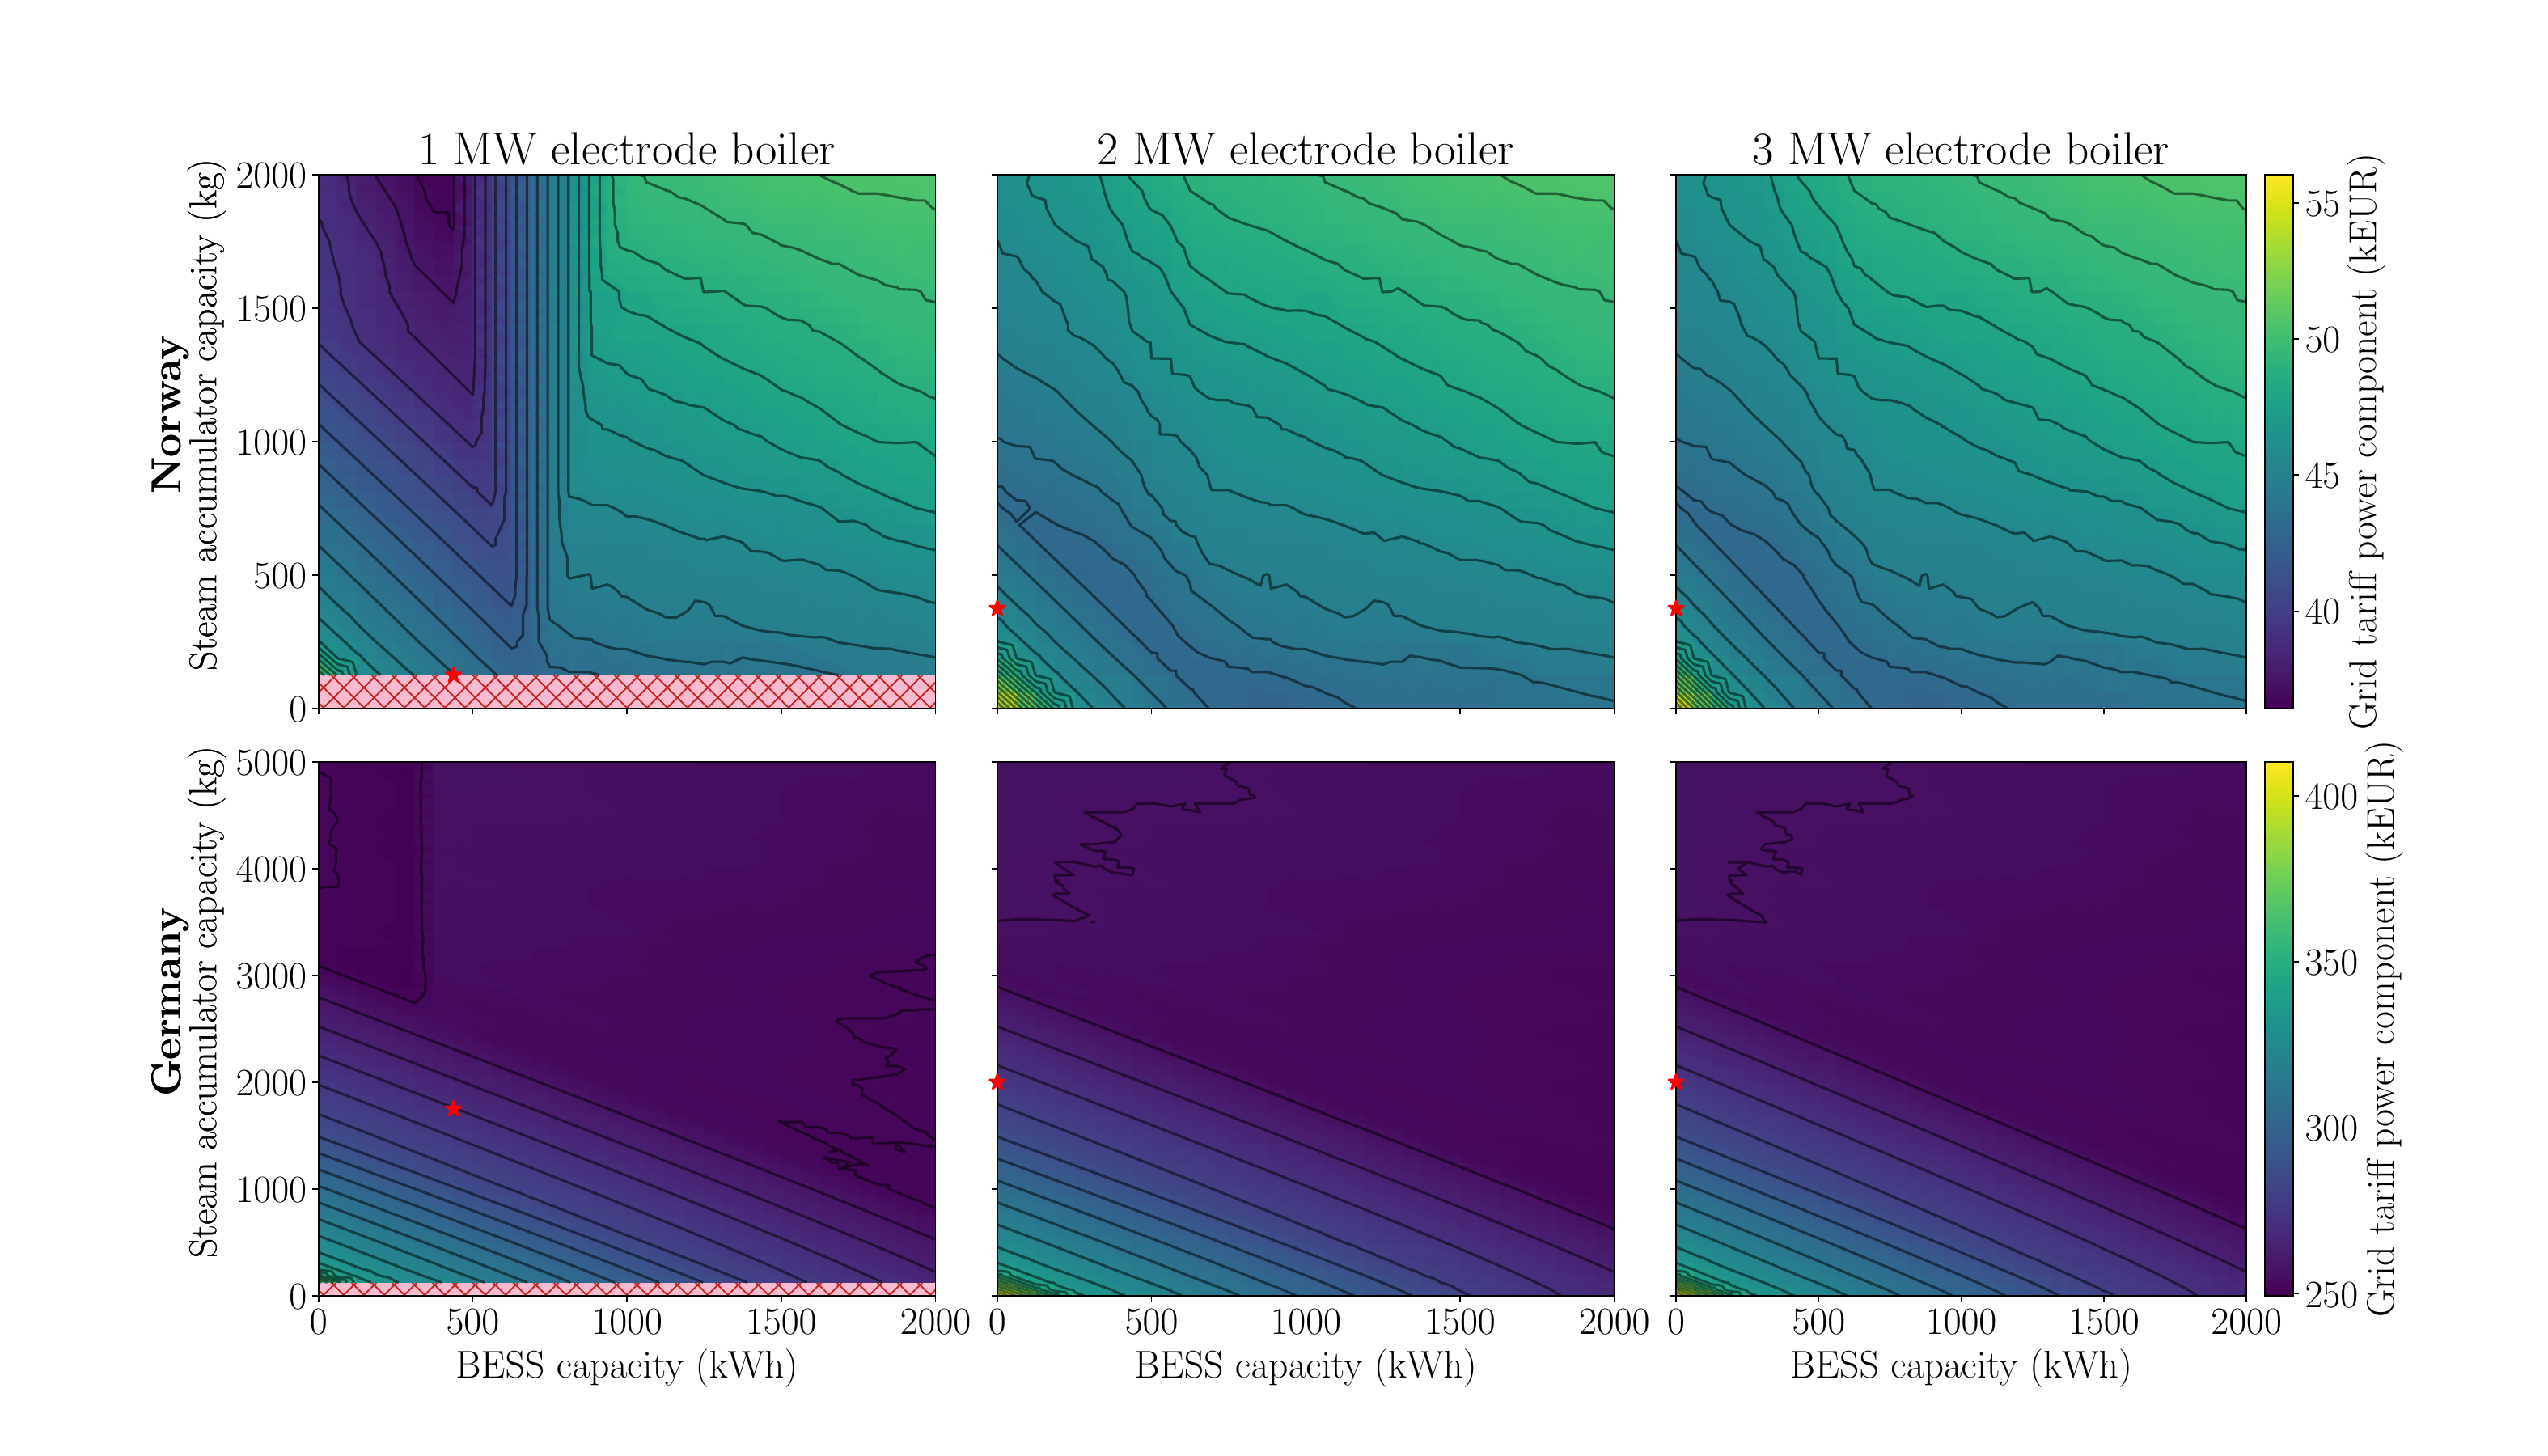}
    \caption{Heat map of the costs from capacity component of the grid tariff for Norway (top) and Germany (bottom) as a function of steam accumulator mass capacity and BESS capacity for three different electrode boiler capacities, (a) \SI{1}{\mega\watt}, (b) \SI{2}{\mega\watt}, an (c) \SI{3}{\mega\watt}. The red star indicates the maximum net present value for each capacity of electrode boiler.}
\end{figure}

\begin{figure}
    \centering
    \includegraphics[width=\linewidth]{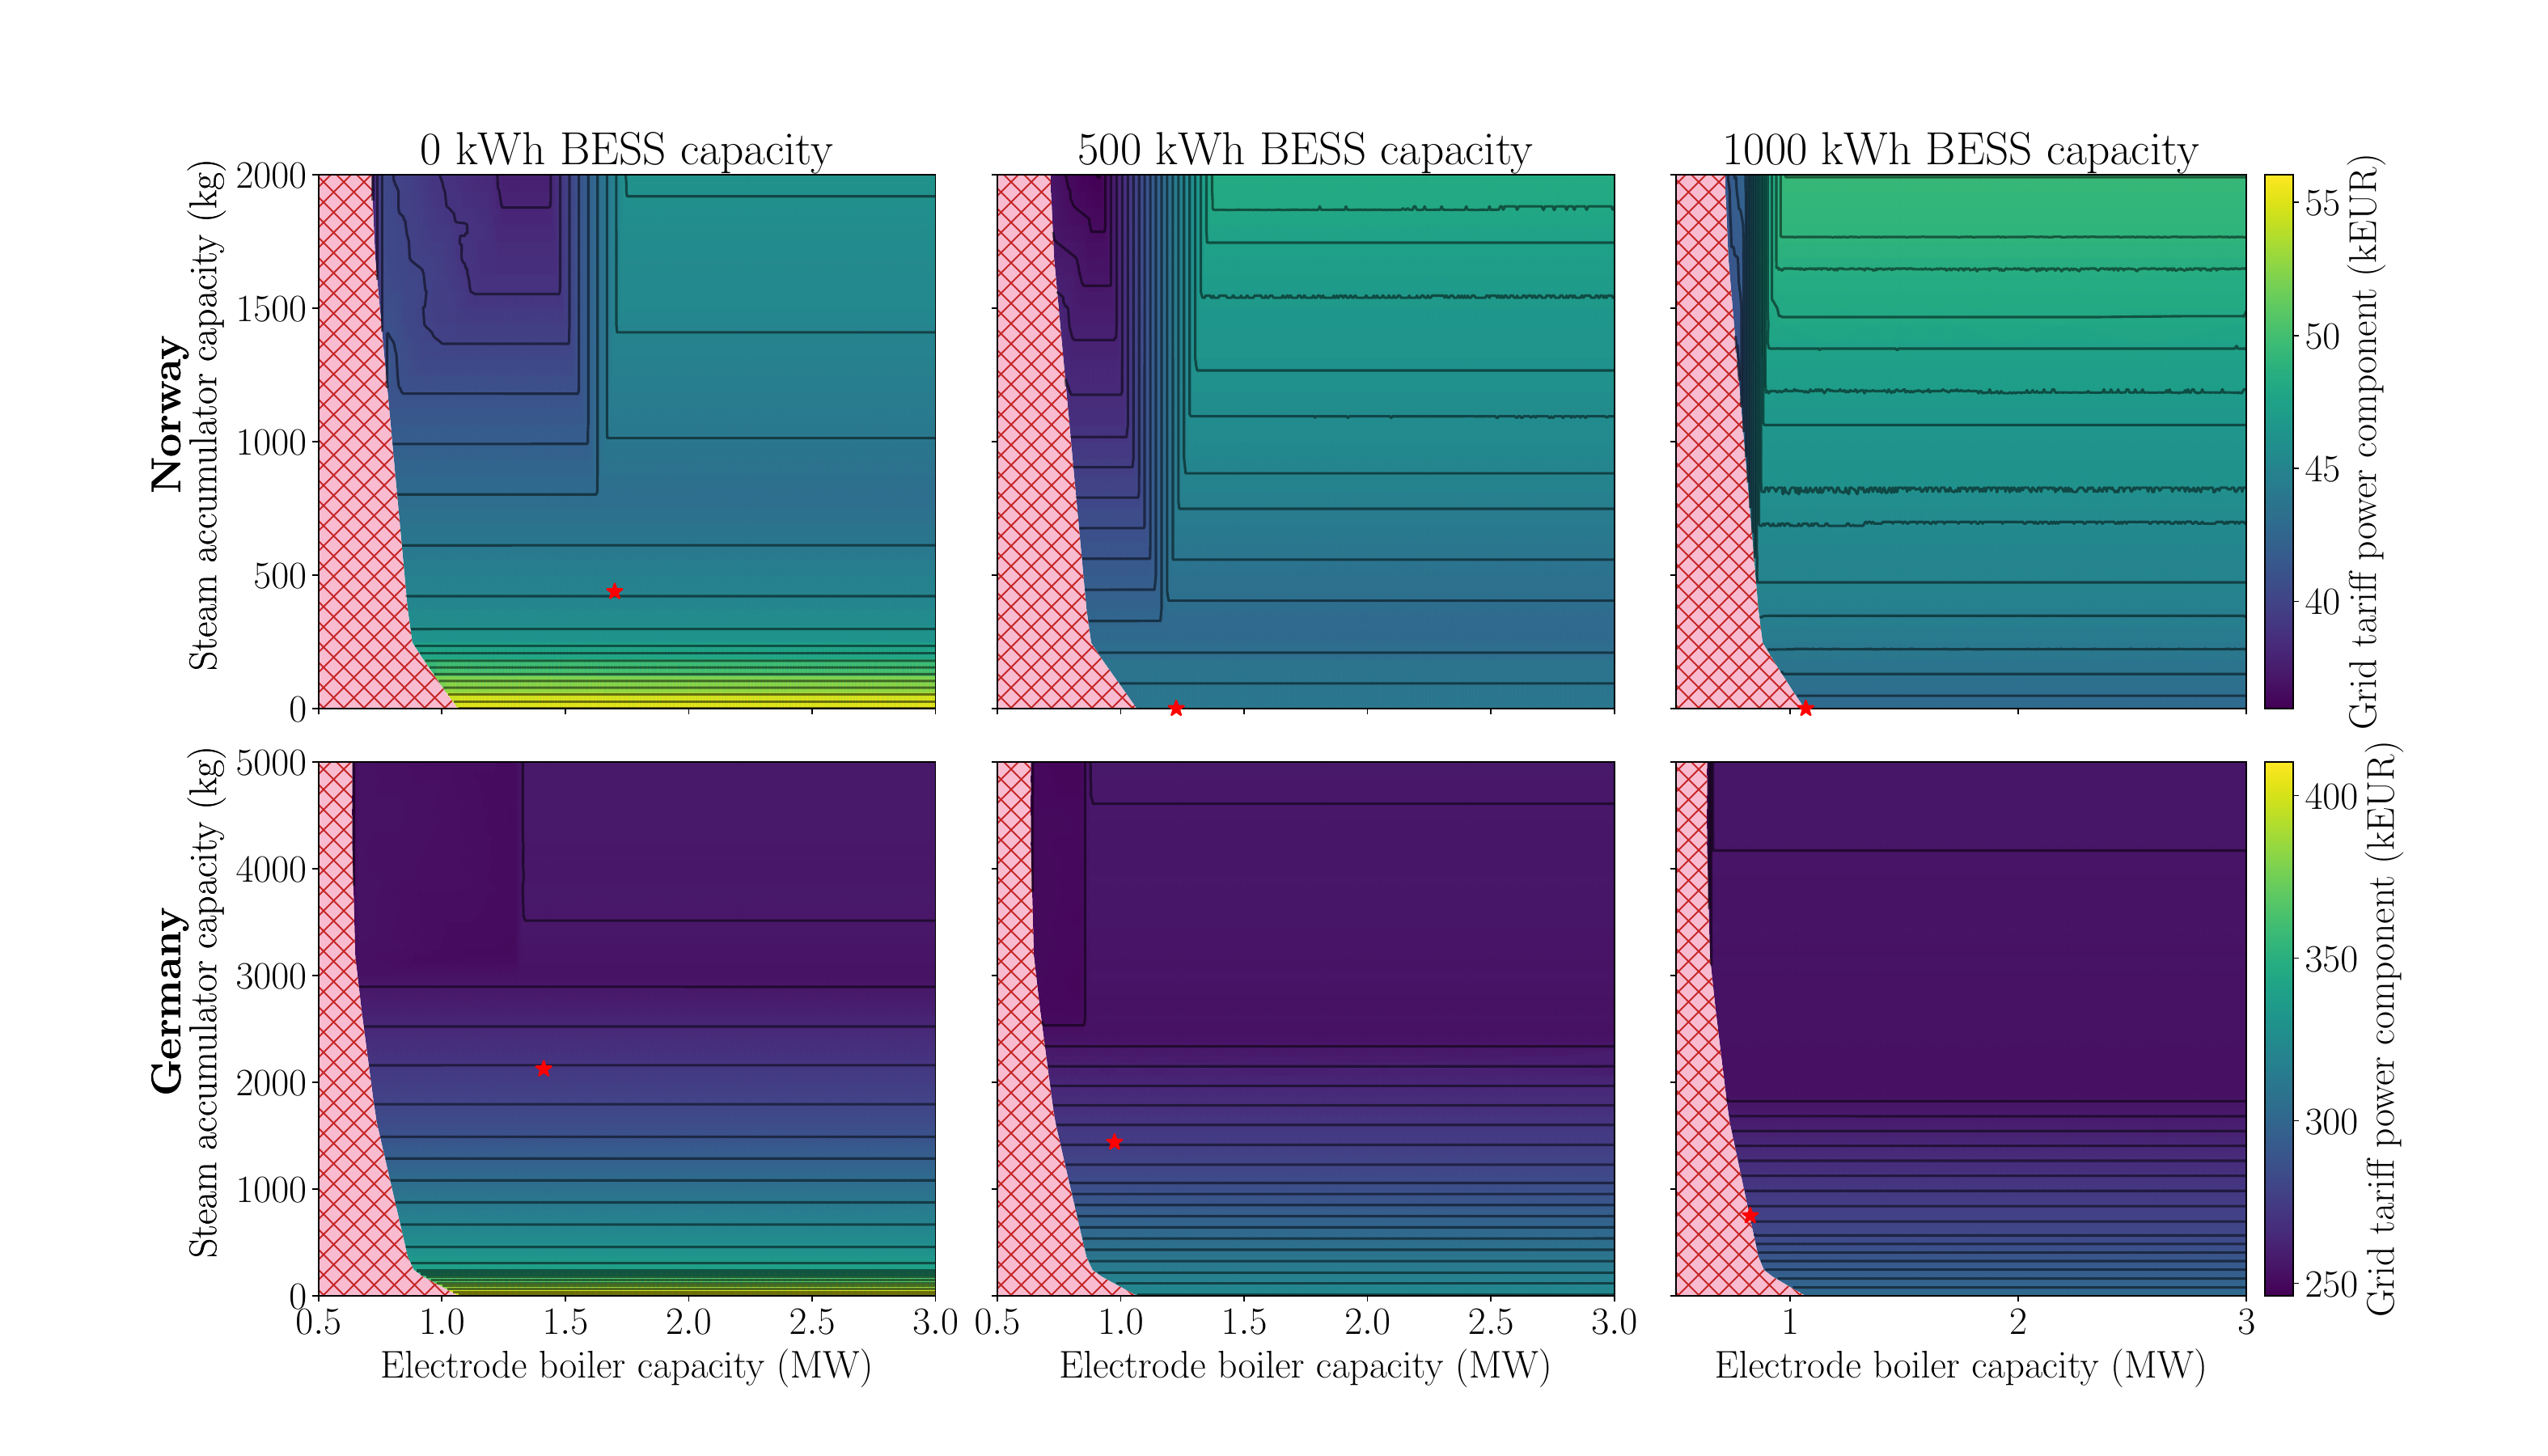}
    \caption{Heat map of the costs from capacity component of the grid tariff for Norway (top) and Germany (bottom) as a function of steam accumulator mass capacity and electrode boiler for three different BESS capacities, (a) \SI{0}{\kilo\Wh}, (b) \SI{500}{\kilo\Wh}, an (c) \SI{1000}{\kilo\Wh} and C-rate of 0.9. The red star indicates the maximum net present value for each capacity of electrode boiler.}
\end{figure}

\begin{figure}
    \centering
    \includegraphics[width=\linewidth]{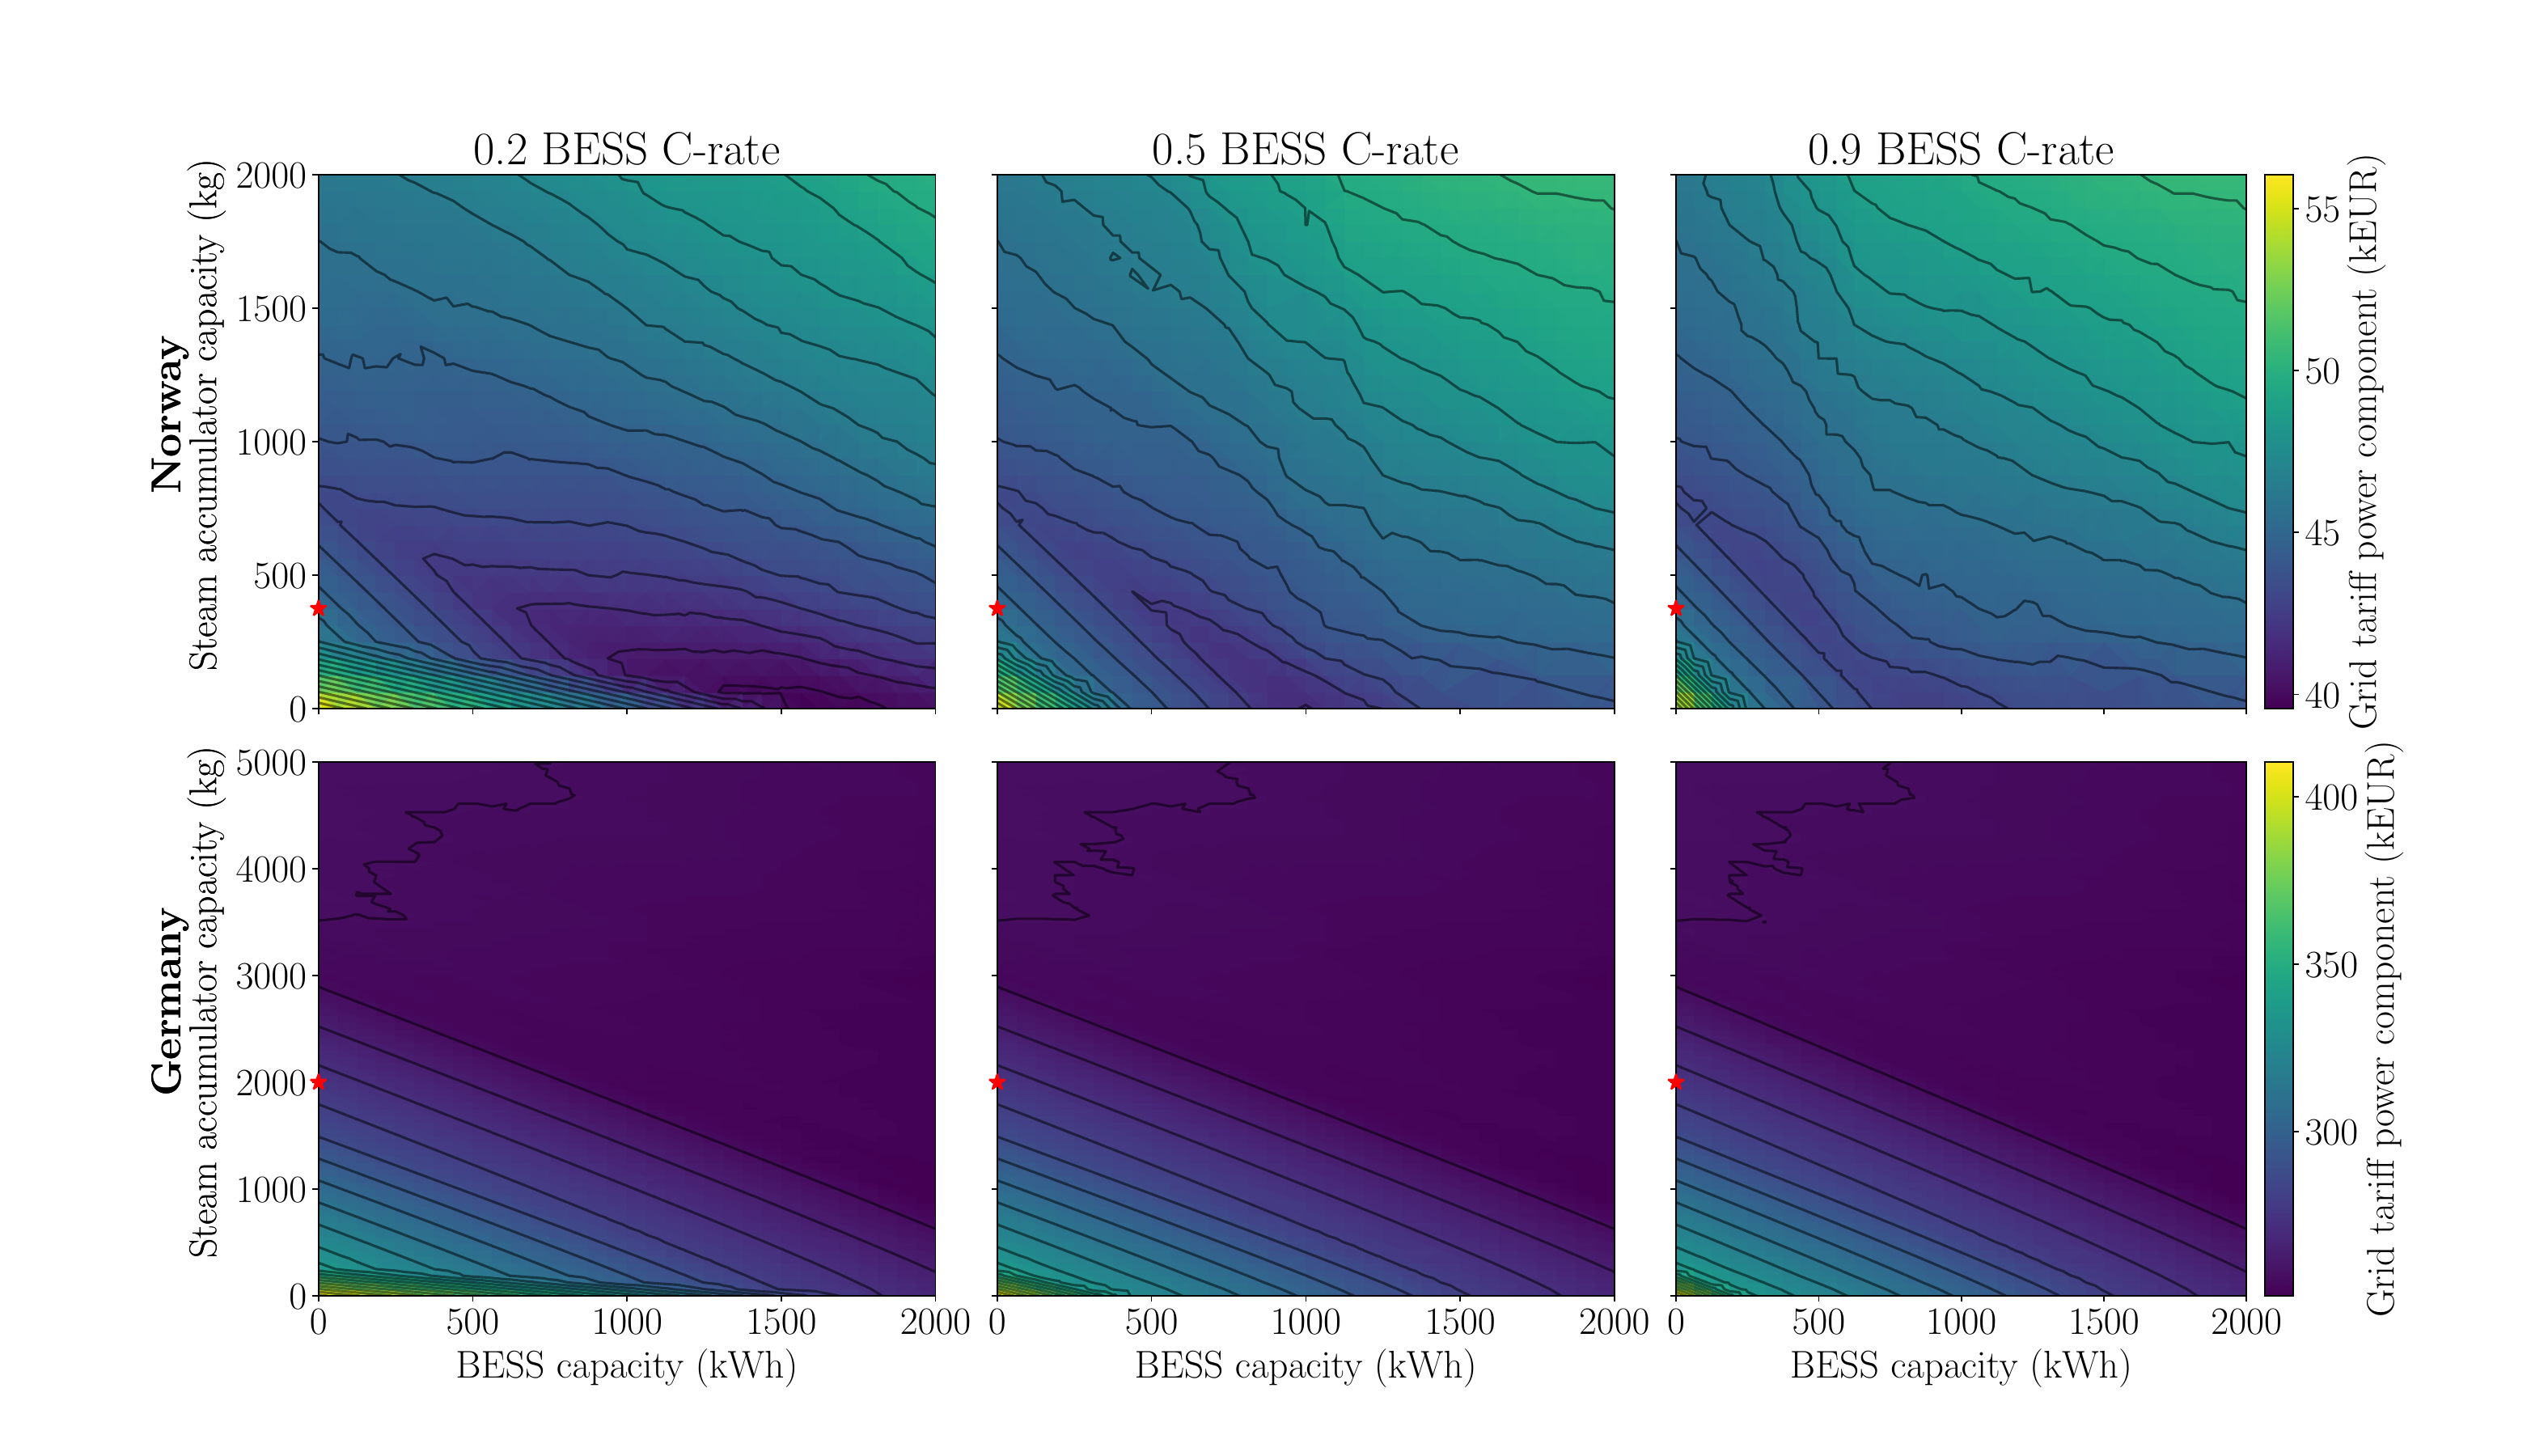}
    \caption{Heat map of the costs from capacity component of the grid tariff for Norway (top) and Germany (bottom) as a function of steam accumulator mass capacity and BESS capacity for electrode boiler capacity of \SI{2}{\mega\watt} and three different BESS C-rates (a) 0.2, (b) 0.5, and (c) 1. The red star indicates the maximum net present value for each capacity of electrode boiler.}
\end{figure}

\begin{figure}
    \centering
    \includegraphics[width=\linewidth]{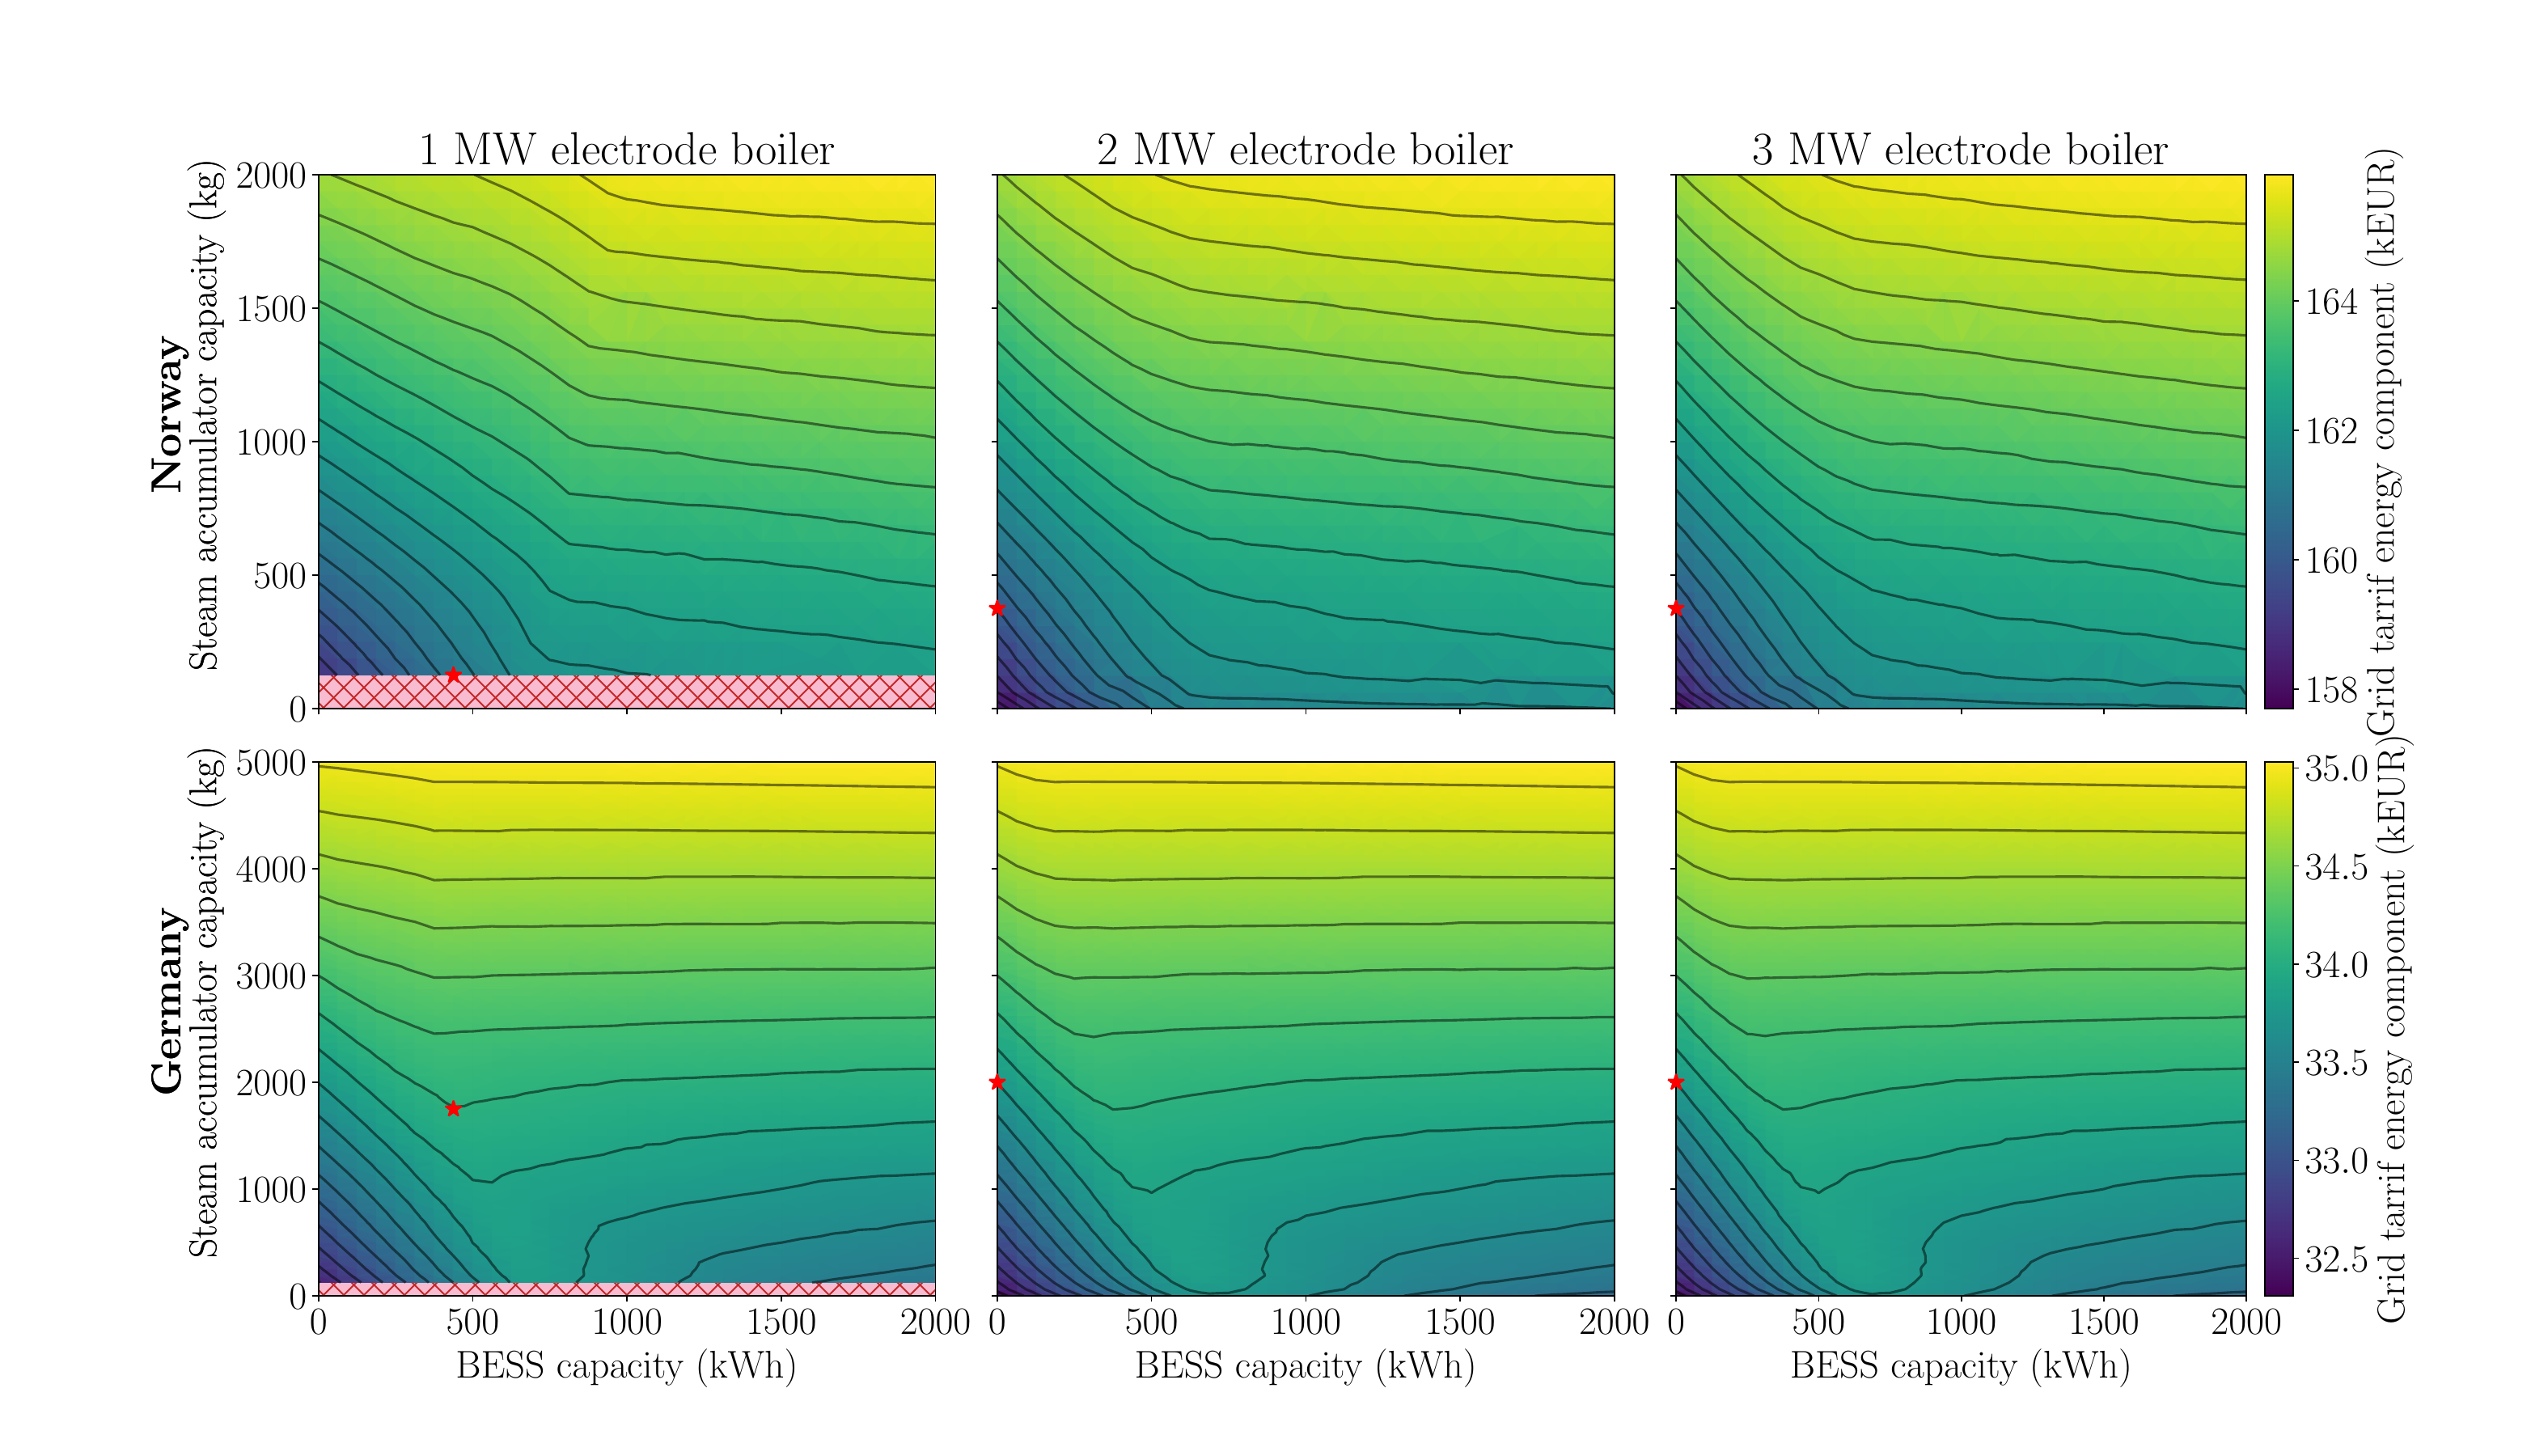}
    \caption{Heat map of the costs from volumetric component of the grid tariff for Norway (top) and Germany (bottom) as a function of steam accumulator mass capacity and BESS capacity for three different electrode boiler capacities, (a) \SI{1}{\mega\watt}, (b) \SI{2}{\mega\watt}, an (c) \SI{3}{\mega\watt}. The red star indicates the maximum net present value for each capacity of electrode boiler.}
\end{figure}

\begin{figure}
    \centering
    \includegraphics[width=\linewidth]{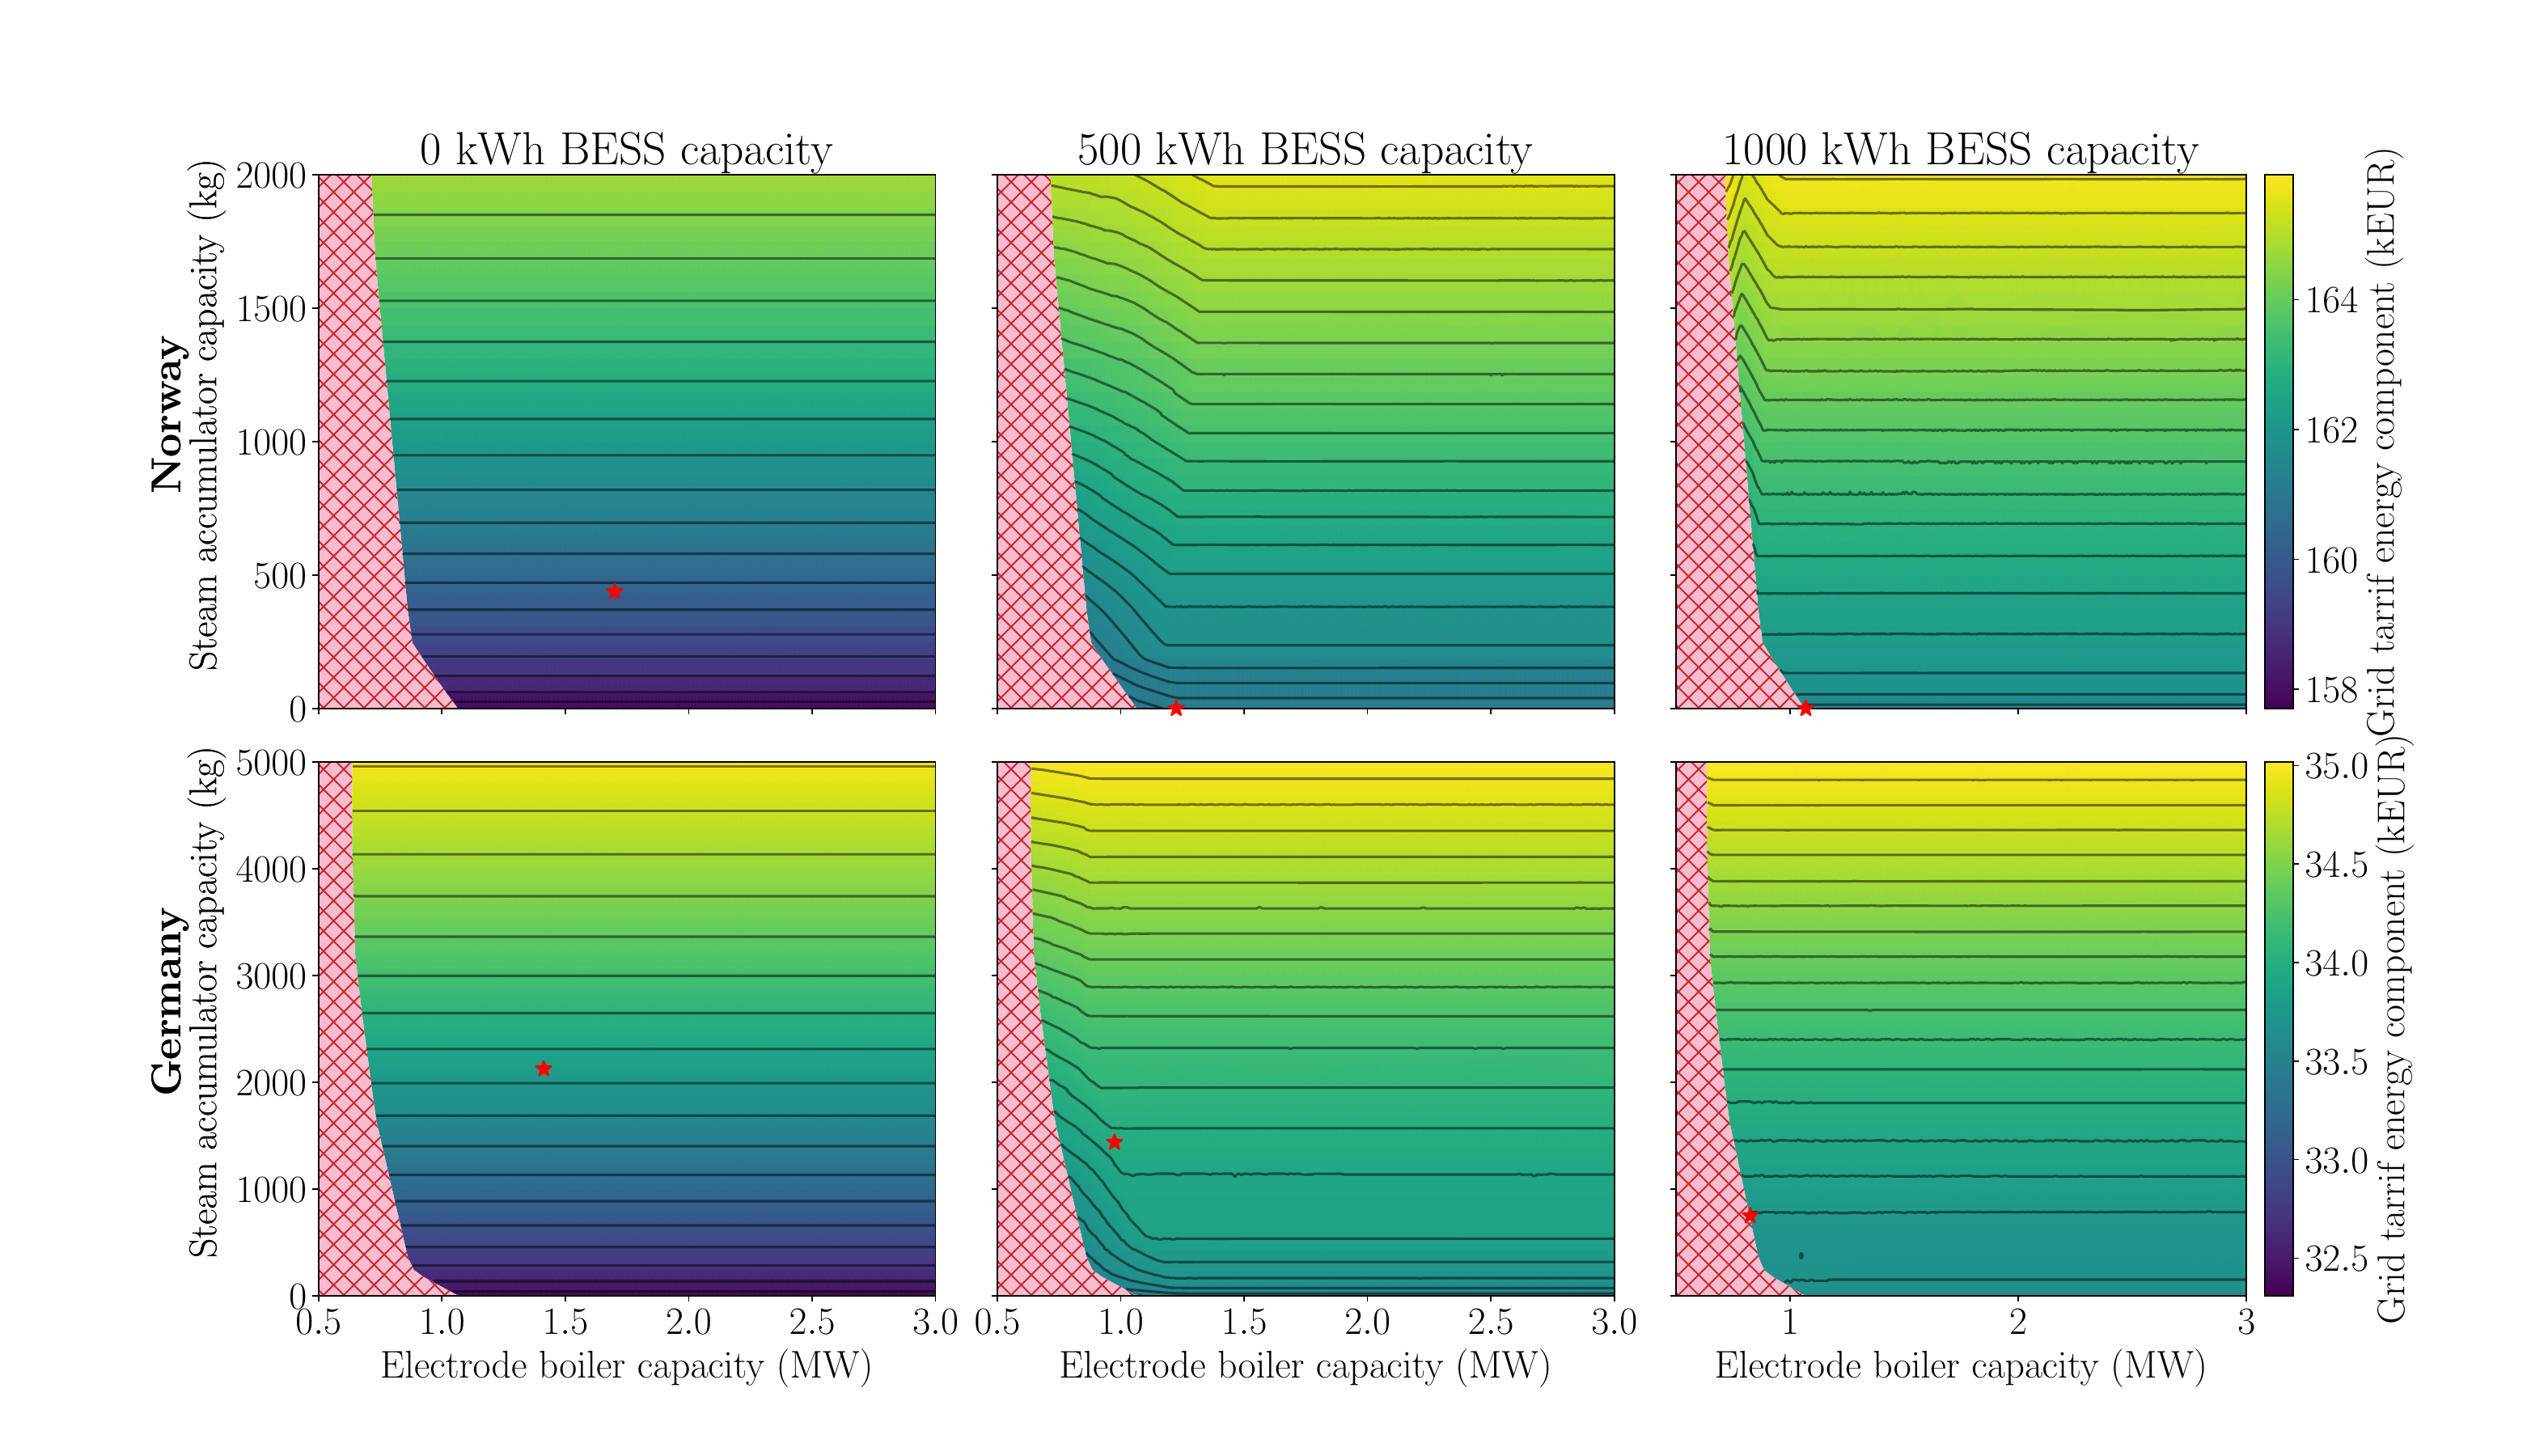}
    \caption{Heat map of the costs from volumetric component of the grid tariff for Norway (top) and Germany (bottom) as a function of steam accumulator mass capacity and electrode boiler for three different BESS capacities, (a) \SI{0}{\kilo\Wh}, (b) \SI{500}{\kilo\Wh}, an (c) \SI{1000}{\kilo\Wh} and C-rate of 0.9. The red star indicates the maximum net present value for each capacity of electrode boiler.}
\end{figure}

\begin{figure}
    \centering
    \includegraphics[width=\linewidth]{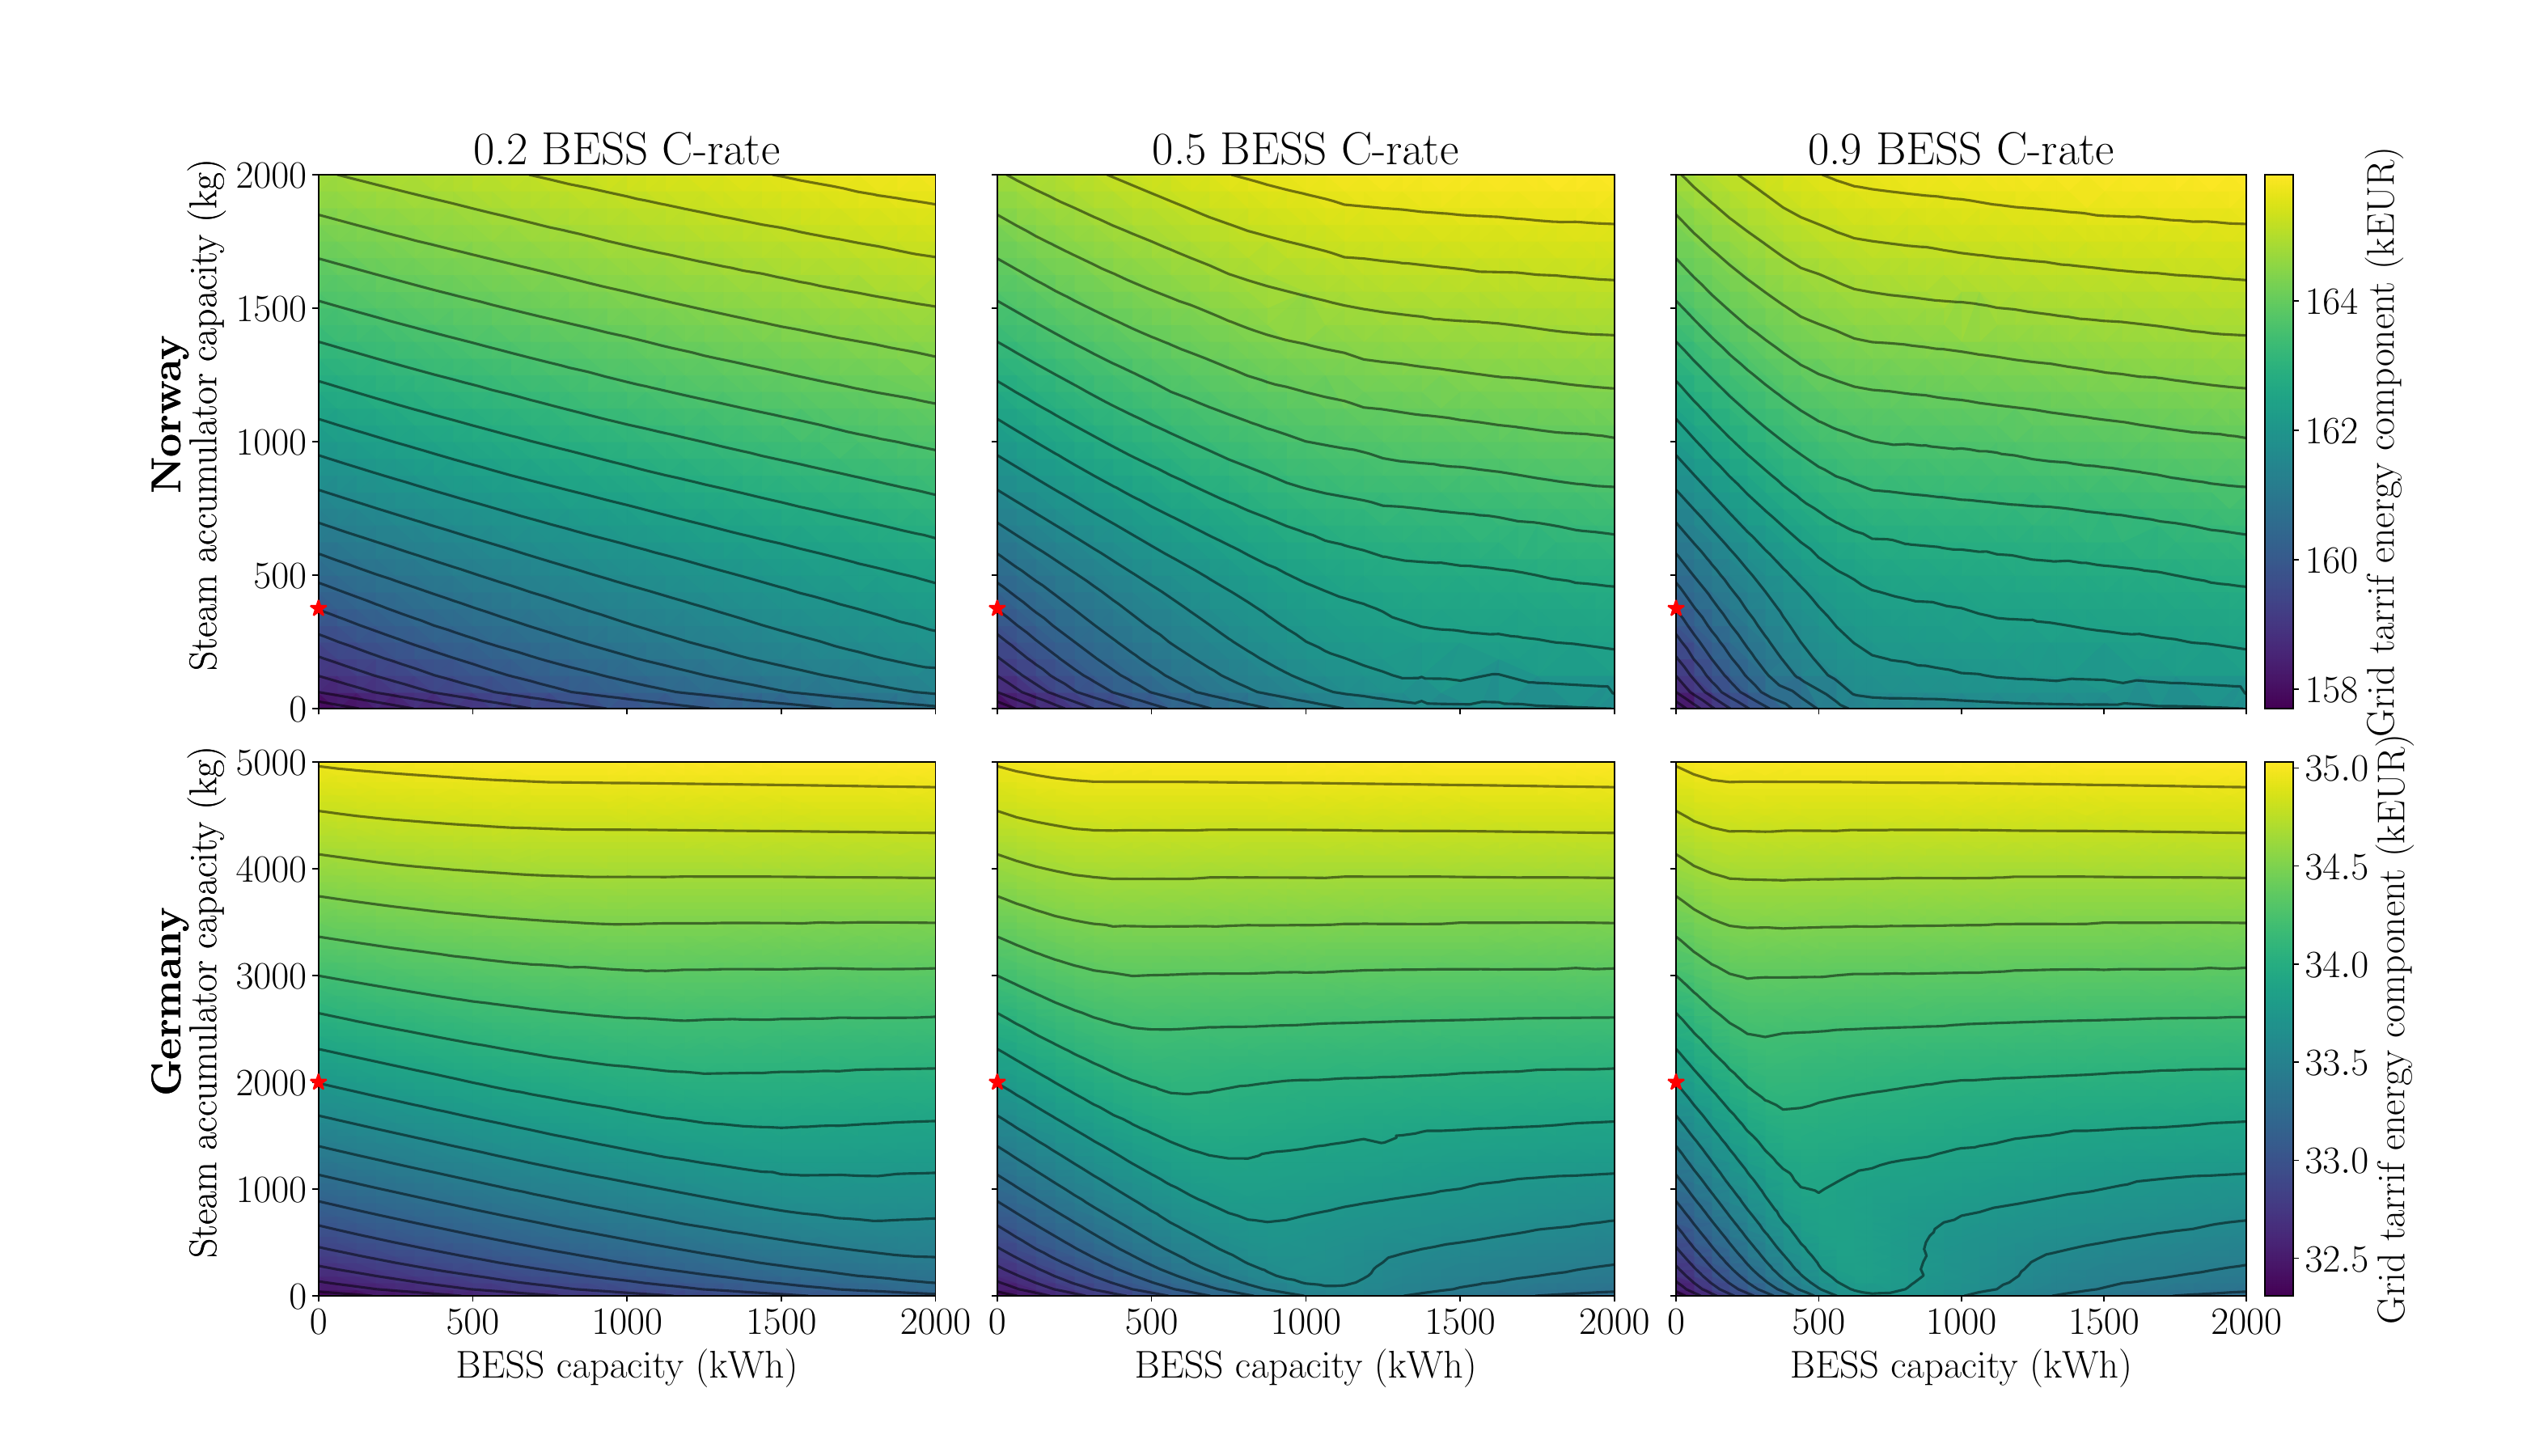}
    \caption{Heat map of the costs from volumetric component of the grid tariff for Norway (top) and Germany (bottom) as a function of steam accumulator mass capacity and BESS capacity for electrode boiler capacity of \SI{2}{\mega\watt} and three different BESS C-rates (a) 0.2, (b) 0.5, and (c) 1. The red star indicates the maximum net present value for each capacity of electrode boiler.}
\end{figure}

\begin{figure}
    \centering
    \includegraphics[width=\linewidth]{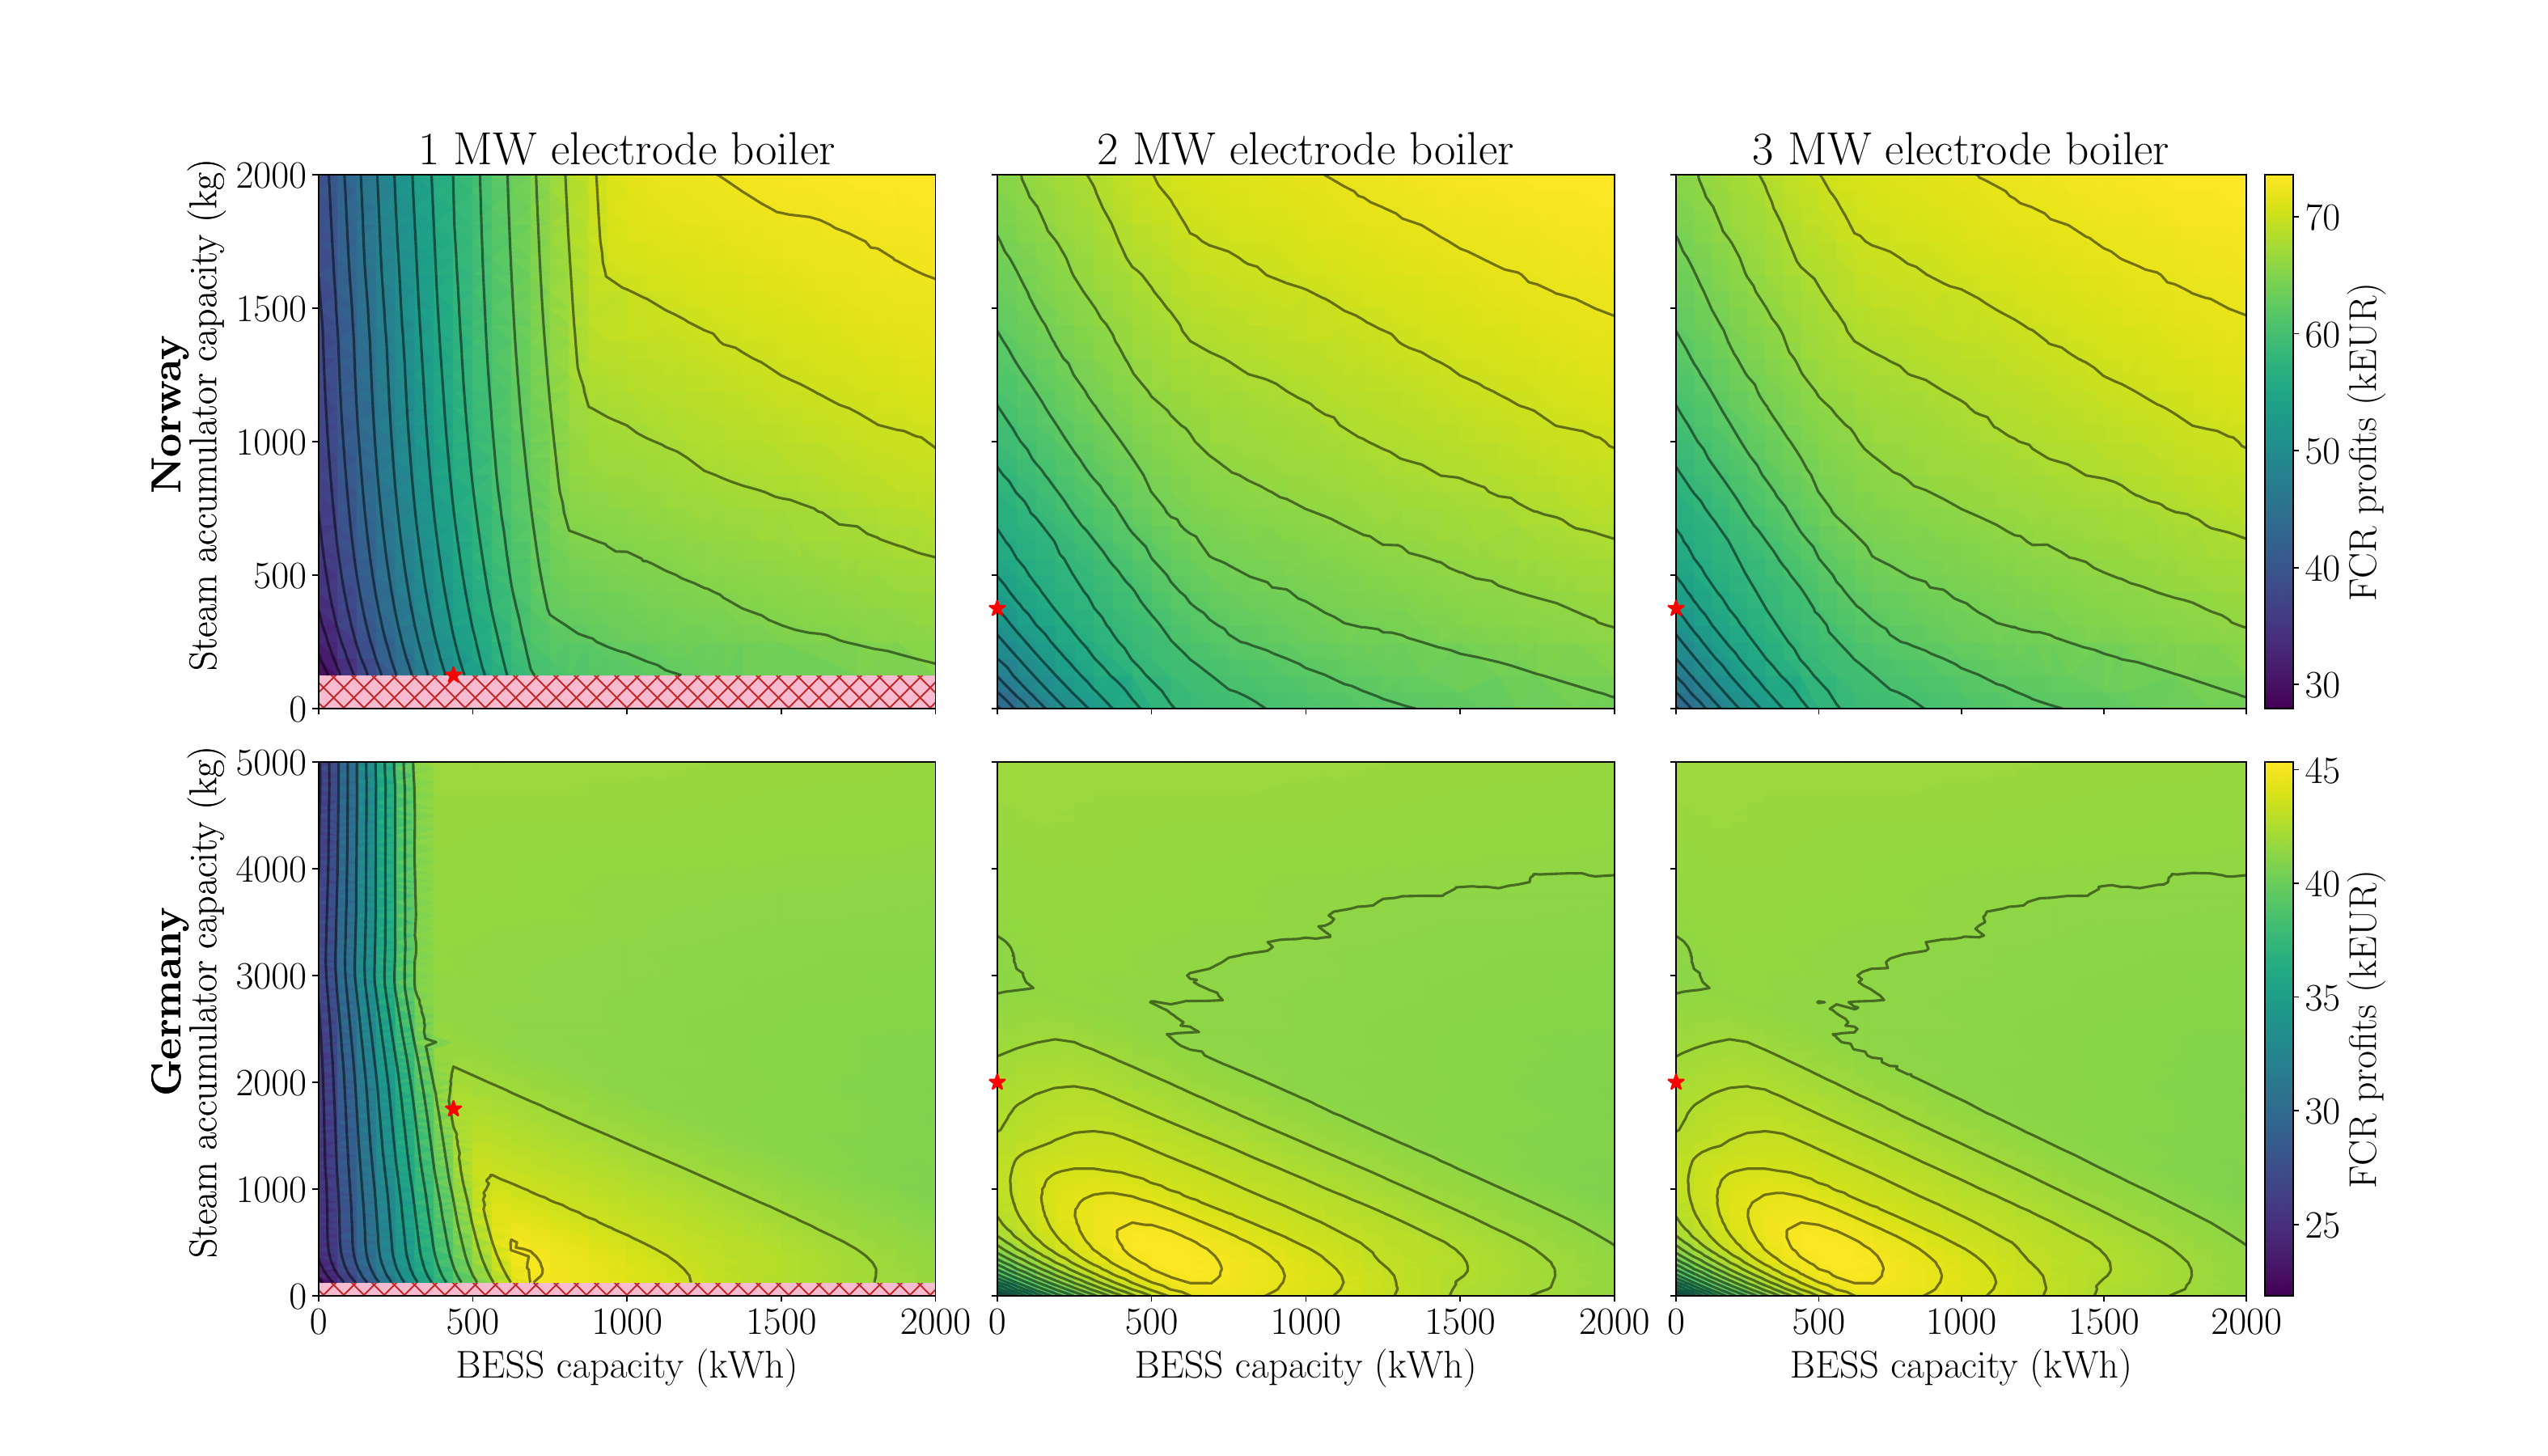}
    \caption{Heat map of the FCR market participation profits for Norway (top) and Germany (bottom) as a function of steam accumulator mass capacity and BESS capacity for three different electrode boiler capacities, (a) \SI{1}{\mega\watt}, (b) \SI{2}{\mega\watt}, an (c) \SI{3}{\mega\watt}. The red star indicates the maximum net present value for each capacity of electrode boiler.}
\end{figure}

\begin{figure}
    \centering
    \includegraphics[width=\linewidth]{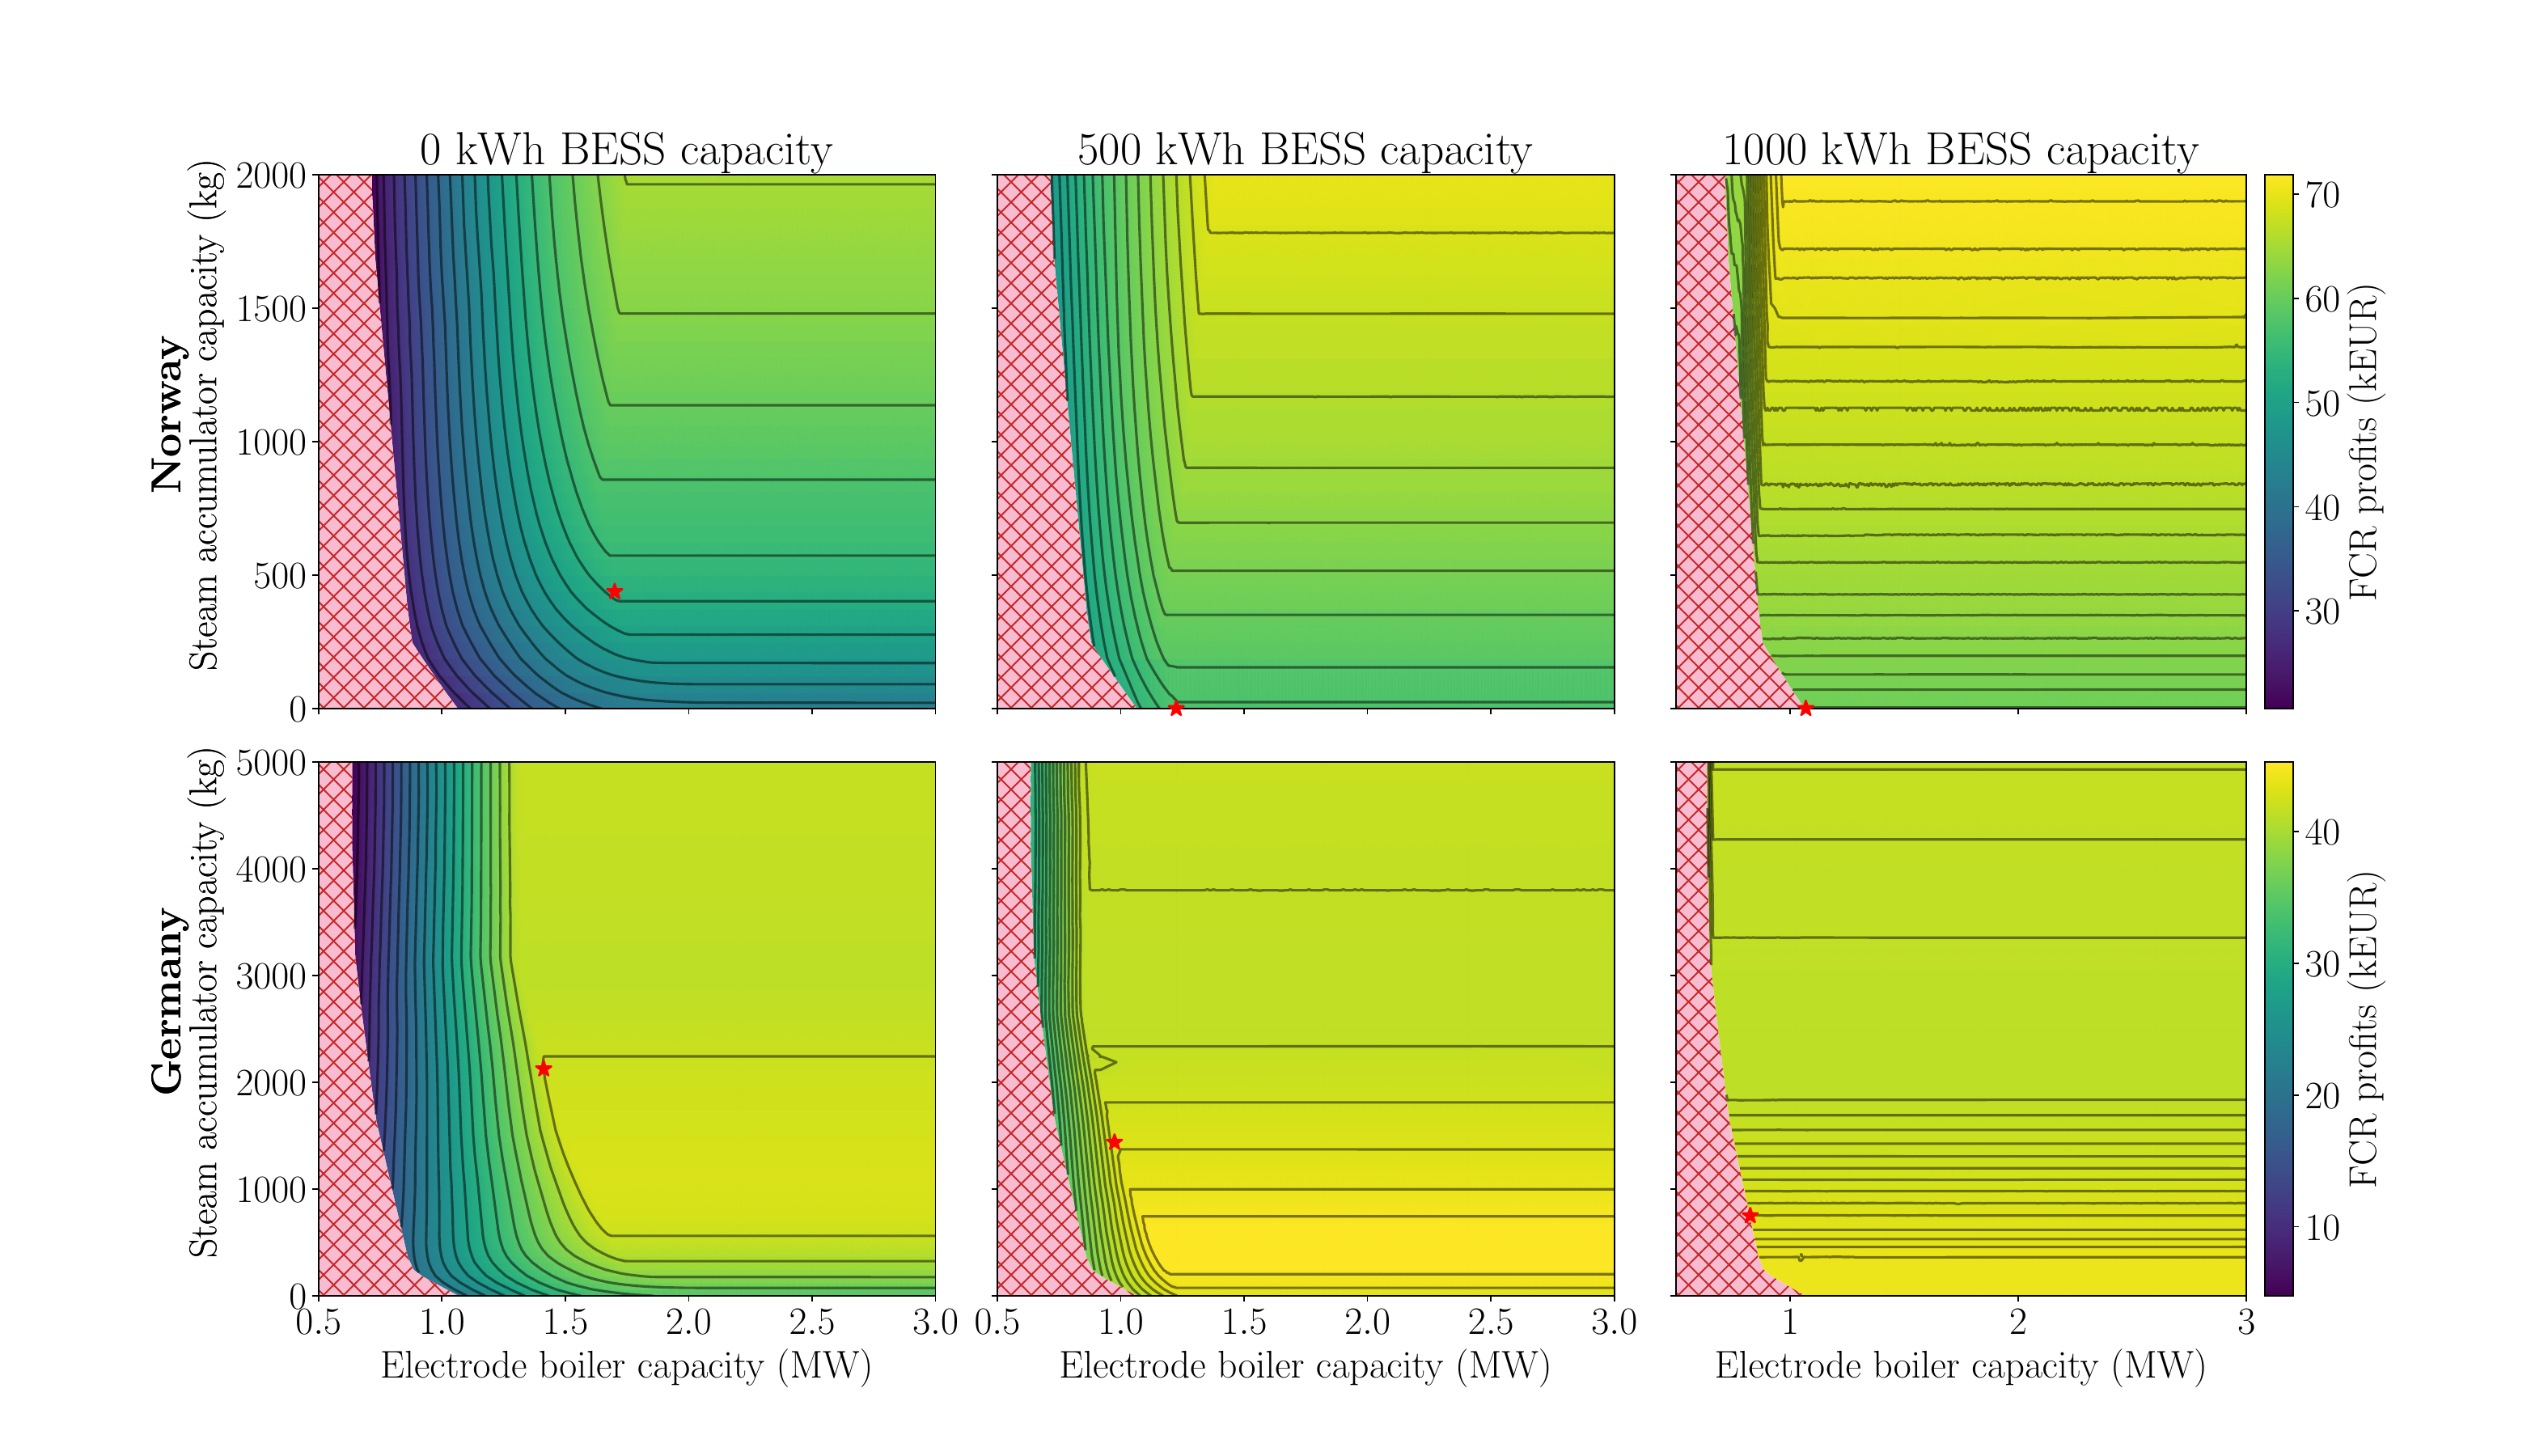}
    \caption{Heat map of the FCR market participation profits for Norway (top) and Germany (bottom) as a function of steam accumulator mass capacity and electrode boiler for three different BESS capacities, (a) \SI{0}{\kilo\Wh}, (b) \SI{500}{\kilo\Wh}, an (c) \SI{1000}{\kilo\Wh} and C-rate of 0.9. The red star indicates the maximum net present value for each capacity of electrode boiler.}
\end{figure}

\begin{figure}
    \centering
    \includegraphics[width=\linewidth]{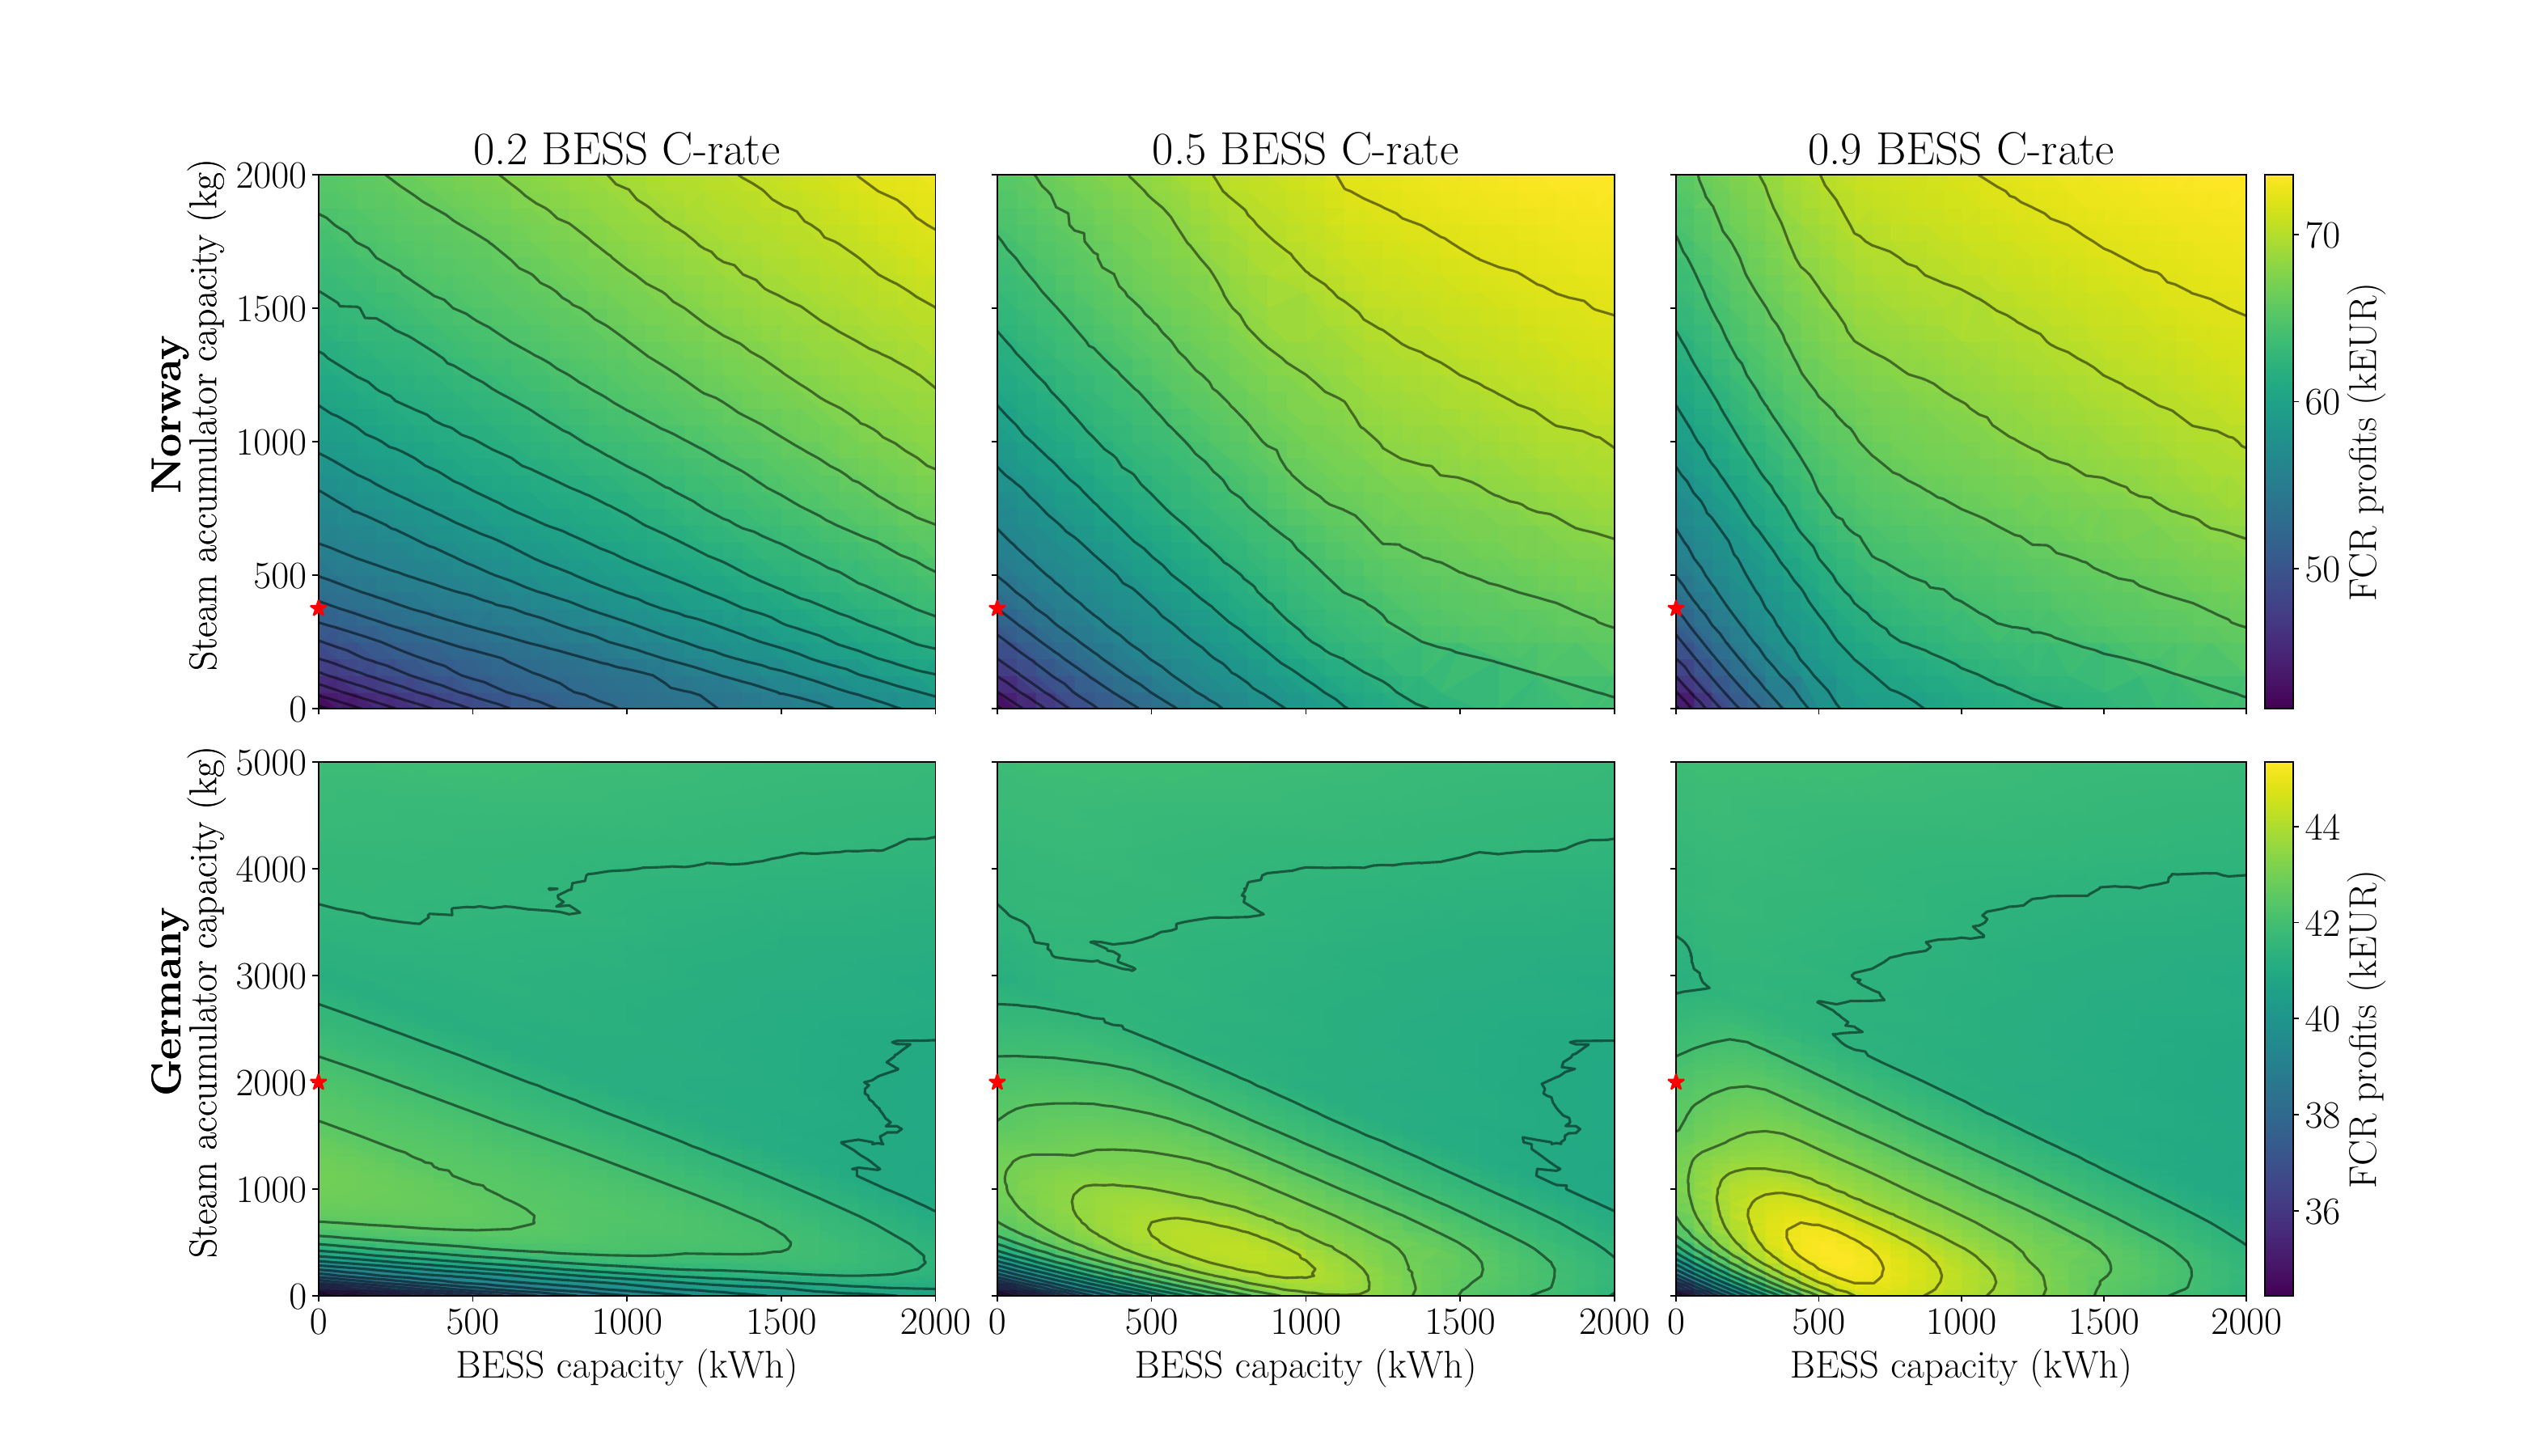}
    \caption{Heat map of the FCR market participation profits for Norway (top) and Germany (bottom) as a function of steam accumulator mass capacity and BESS capacity for electrode boiler capacity of \SI{2}{\mega\watt} and three different BESS C-rates (a) 0.2, (b) 0.5, and (c) 1. The red star indicates the maximum net present value for each capacity of electrode boiler.}
\end{figure}

\begin{figure}
    \centering
    \includegraphics[width=\linewidth]{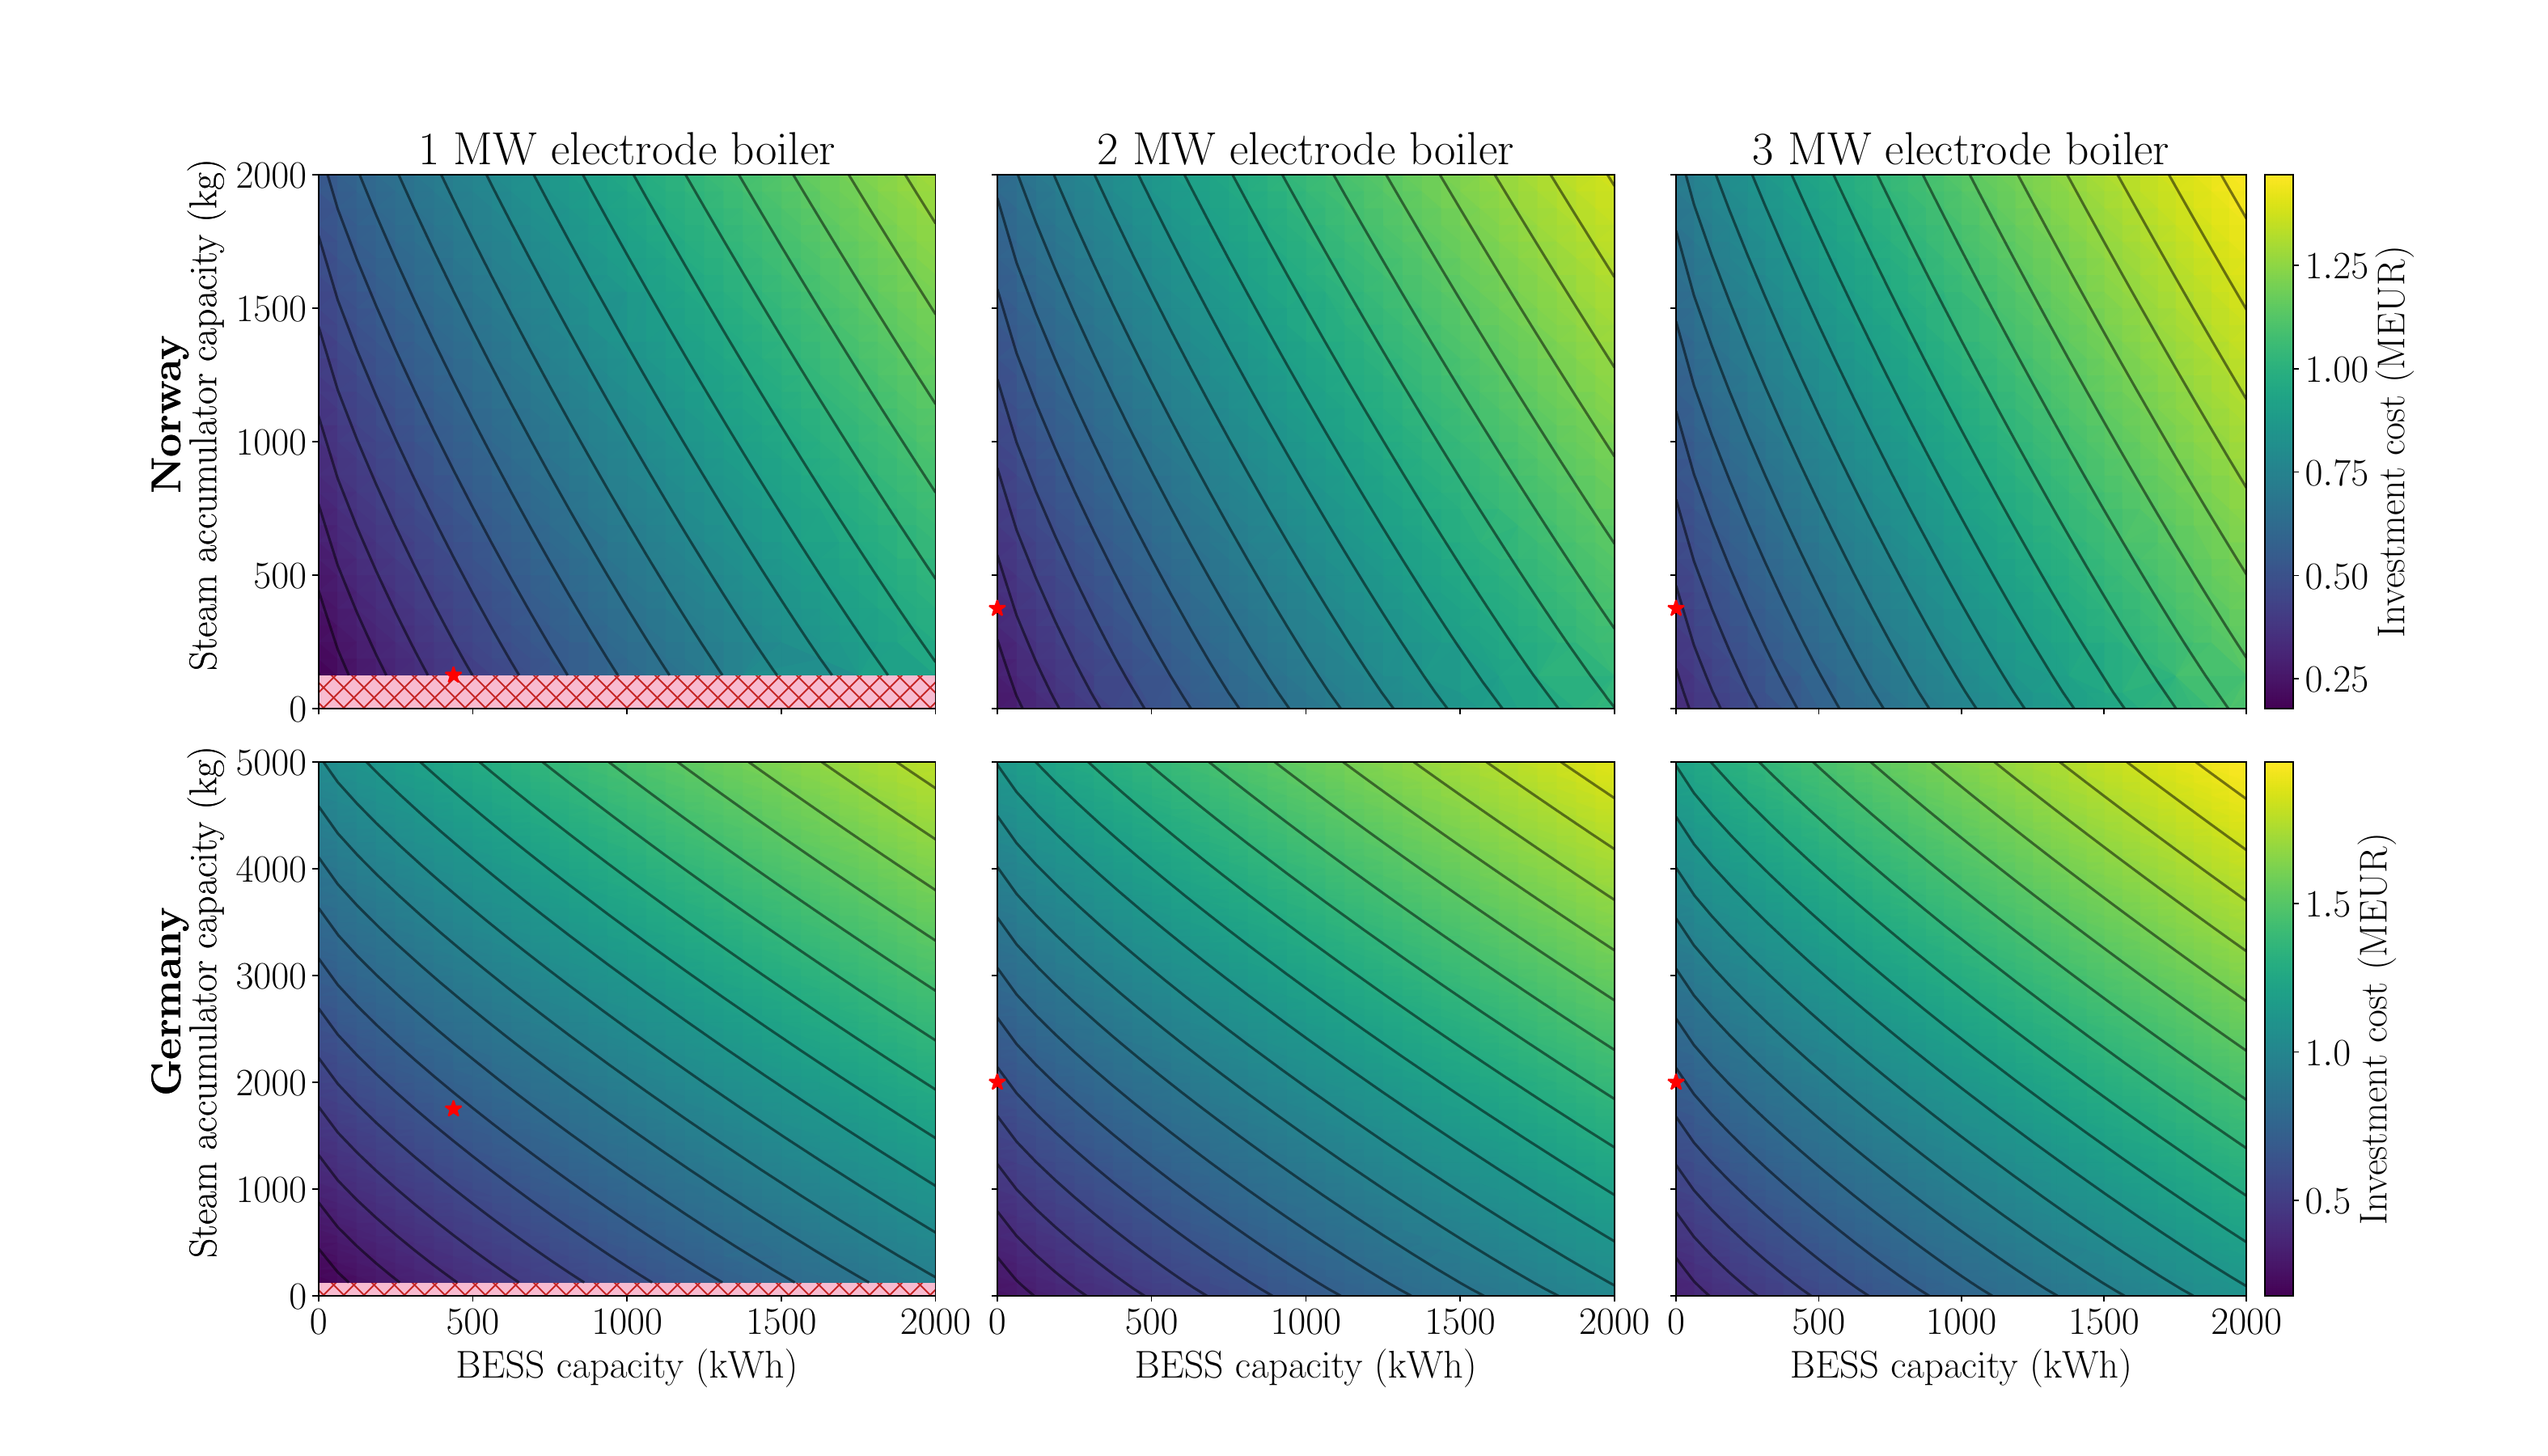}
    \caption{Heat map of the investment costs for Norway (top) and Germany (bottom) as a function of steam accumulator mass capacity and BESS capacity for three different electrode boiler capacities, (a) \SI{1}{\mega\watt}, (b) \SI{2}{\mega\watt}, an (c) \SI{3}{\mega\watt}. The red star indicates the maximum net present value for each capacity of electrode boiler.}
\end{figure}

\begin{figure}
    \centering
    \includegraphics[width=\linewidth]{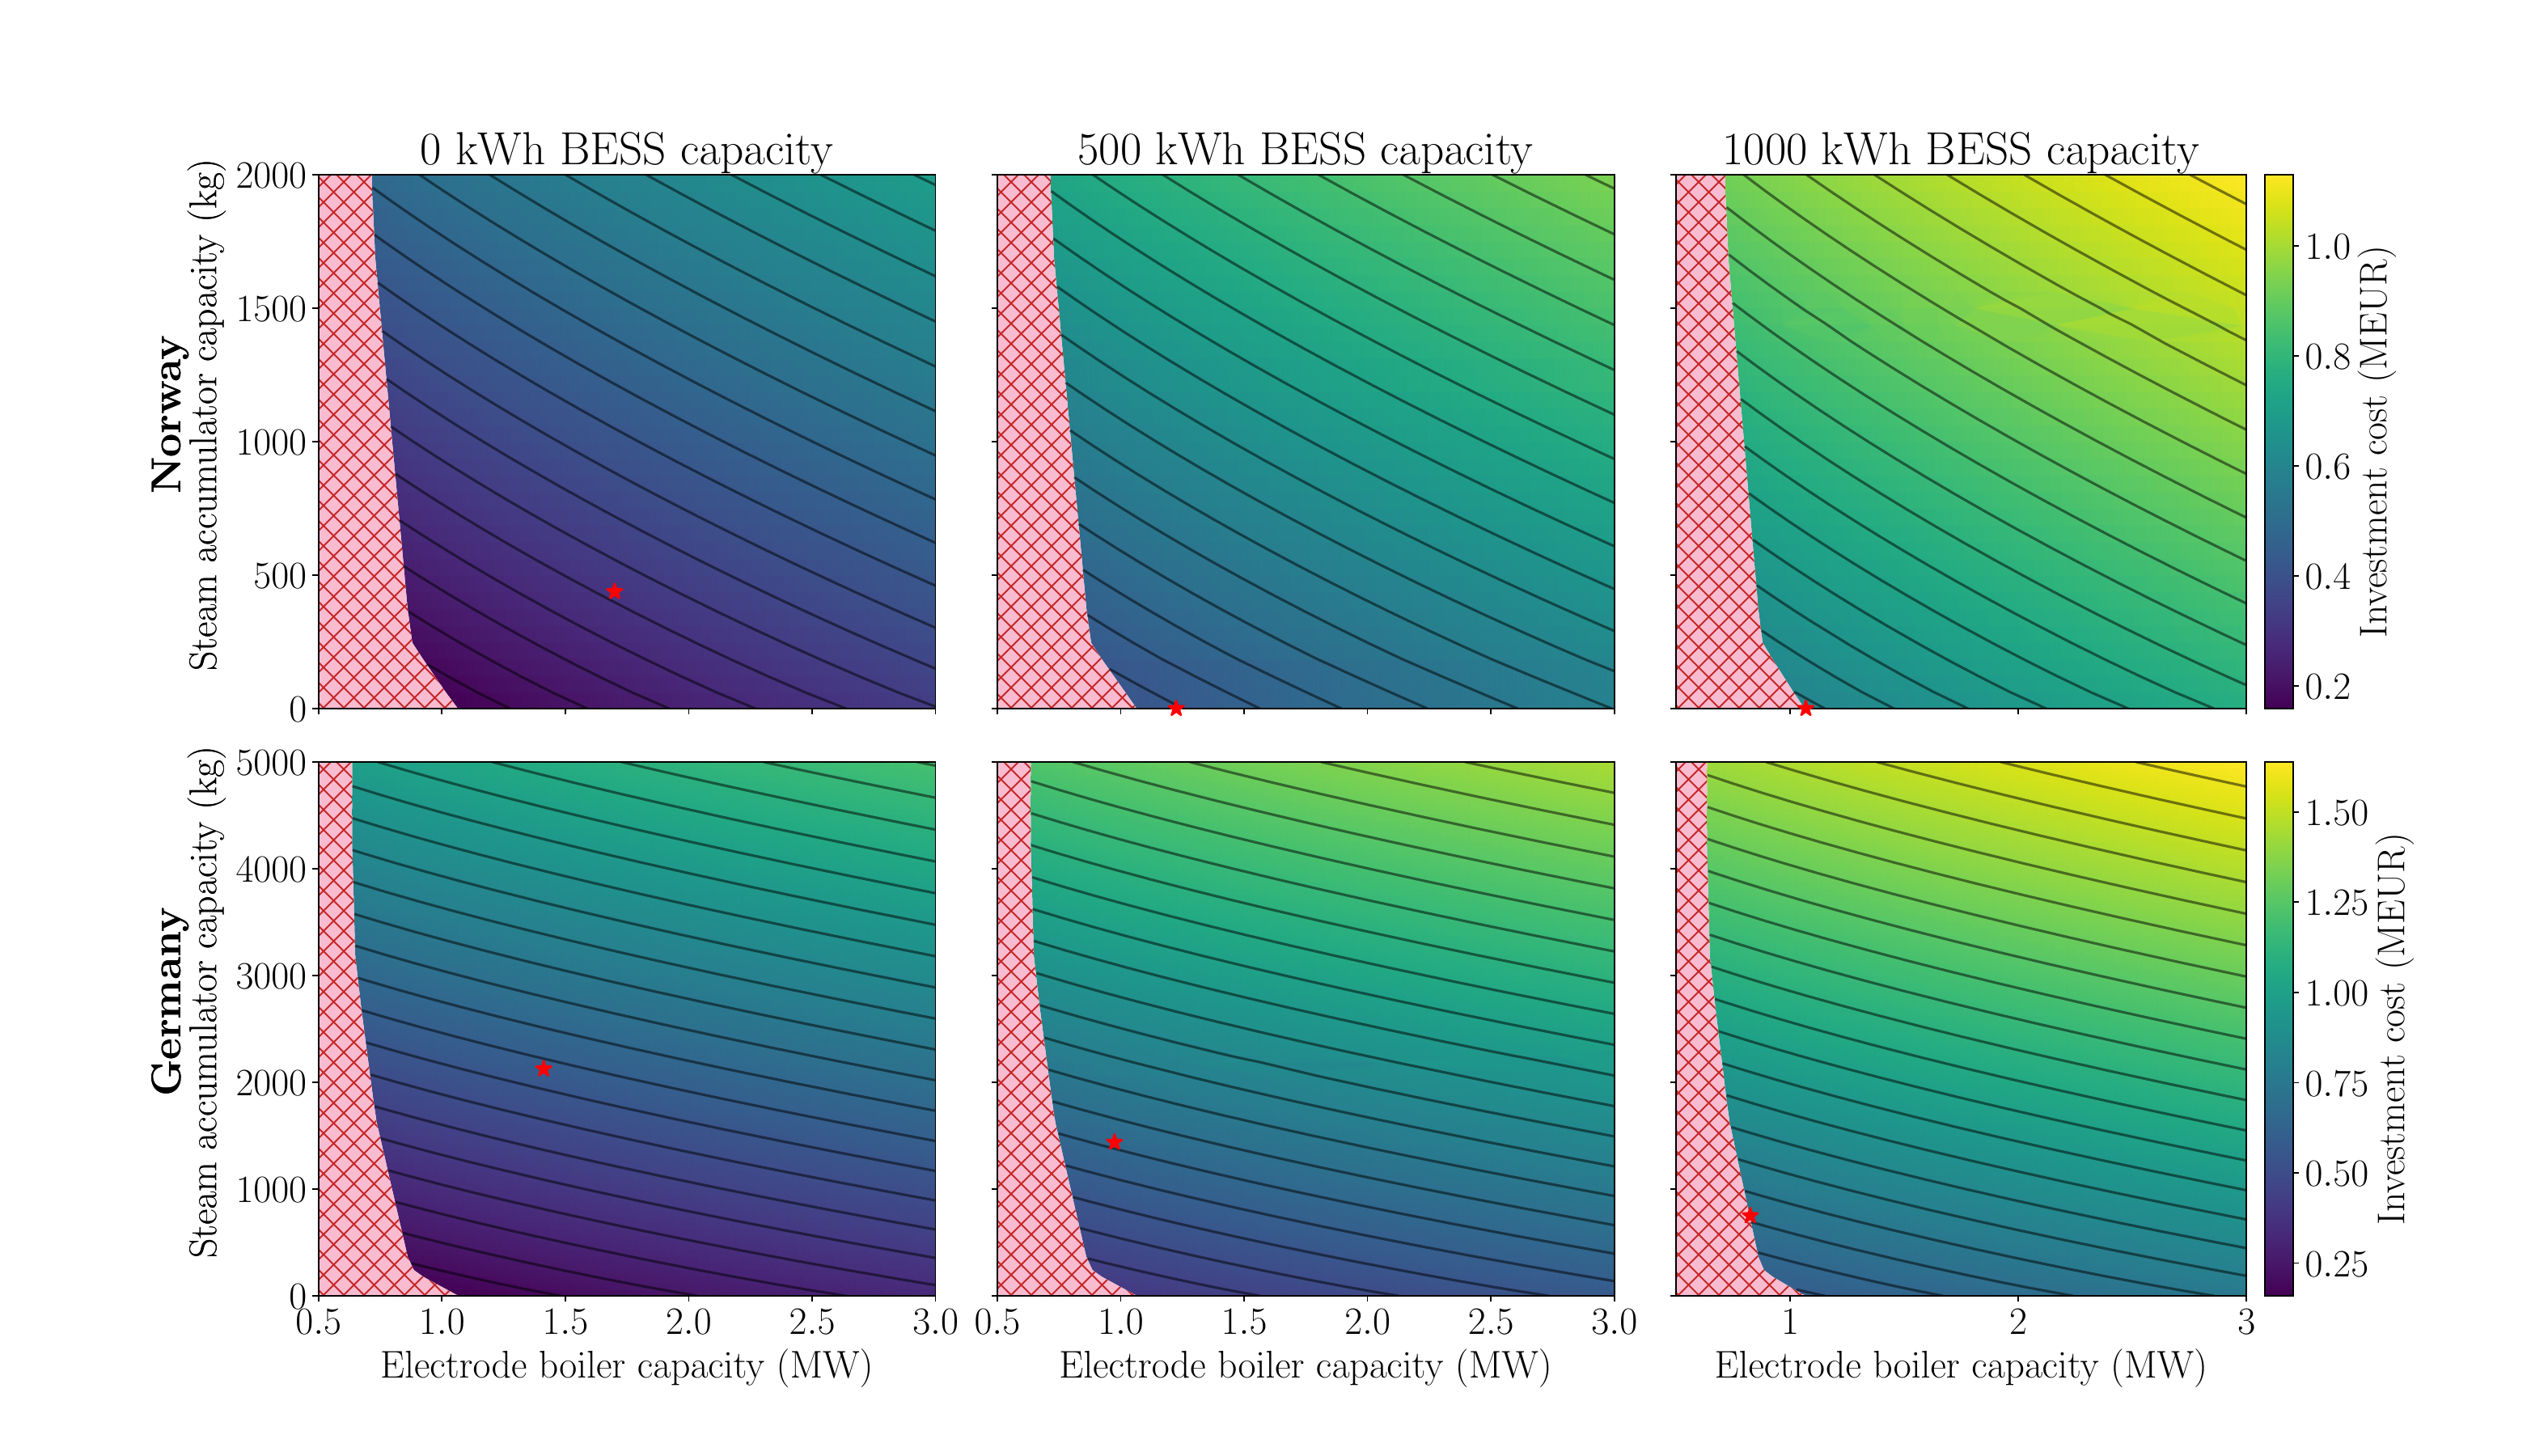}
    \caption{Heat map of the investment costs for Norway (top) and Germany (bottom) as a function of steam accumulator mass capacity and electrode boiler for three different BESS capacities, (a) \SI{0}{\kilo\Wh}, (b) \SI{500}{\kilo\Wh}, an (c) \SI{1000}{\kilo\Wh} and C-rate of 0.9. The red star indicates the maximum net present value for each capacity of electrode boiler.}
\end{figure}

\begin{figure}
    \centering
    \includegraphics[width=\linewidth]{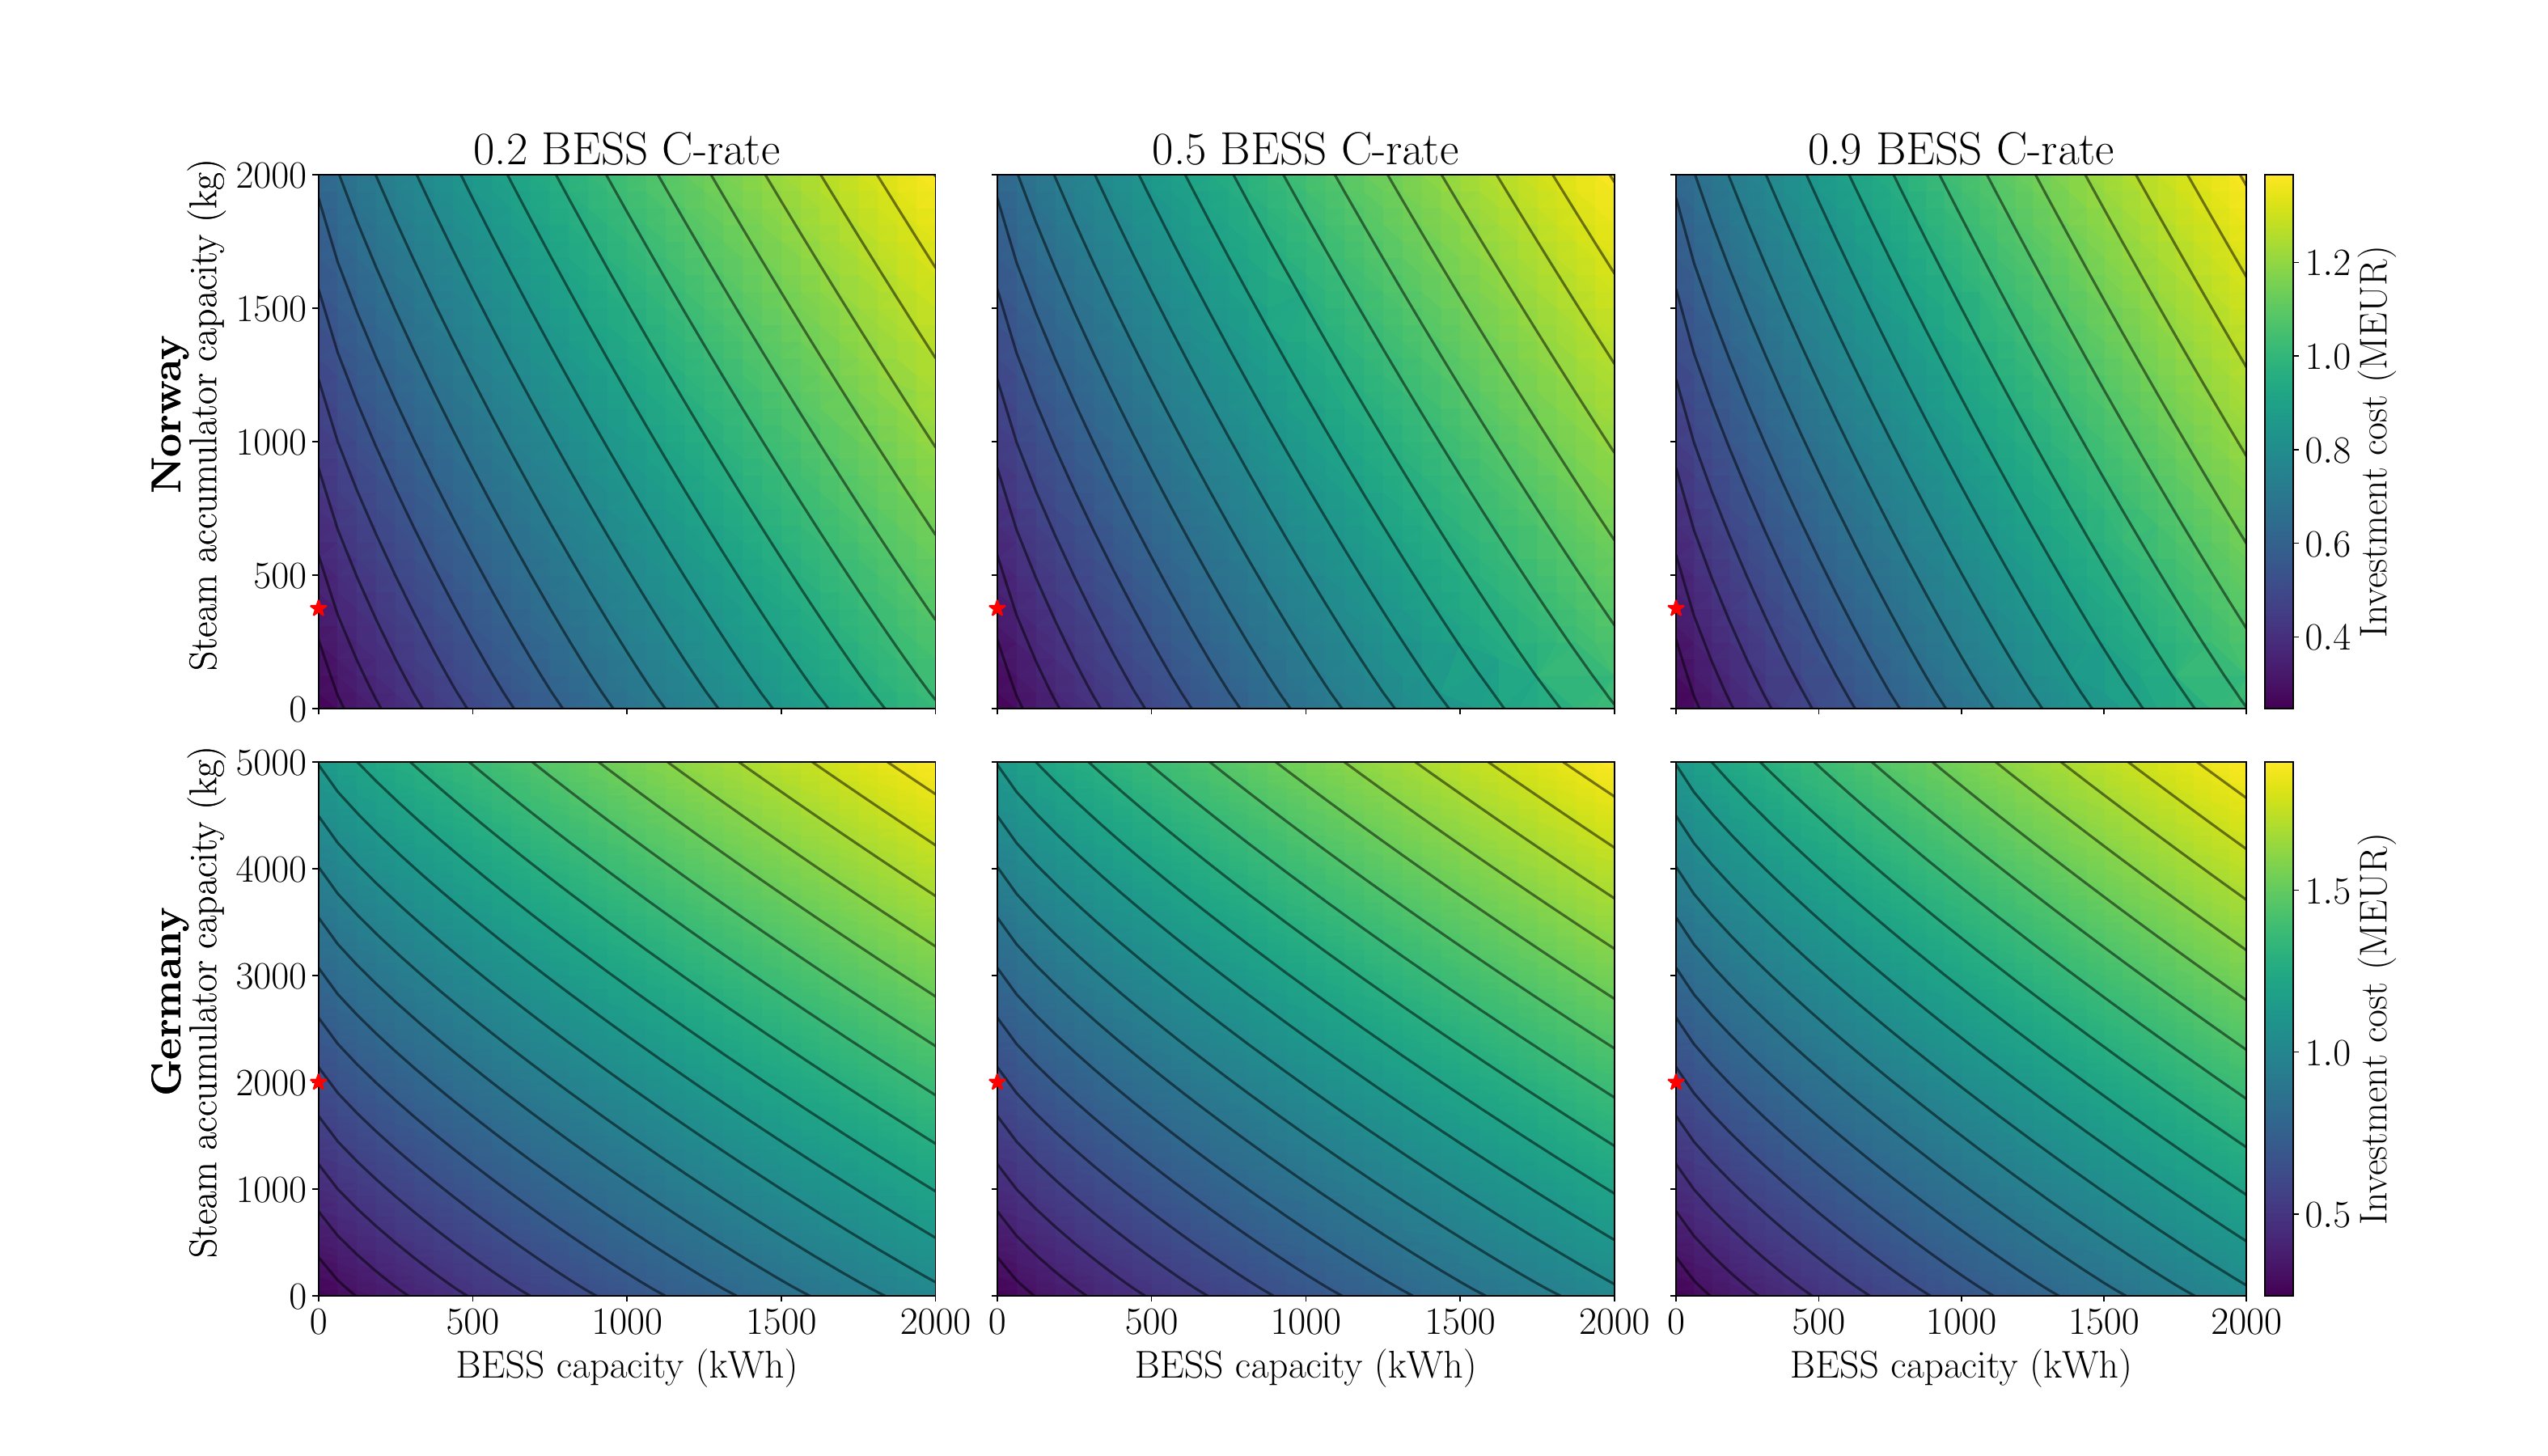}
    \caption{Heat map of the investment costs for Norway (top) and Germany (bottom) as a function of steam accumulator mass capacity and BESS capacity for electrode boiler capacity of \SI{2}{\mega\watt} and three different BESS C-rates (a) 0.2, (b) 0.5, and (c) 1. The red star indicates the maximum net present value for each capacity of electrode boiler.}
\end{figure}
\end{document}
